# Supplementary material for: ChemiRise: a data-driven retrosynthesis engine
Source: arXiv:2108.04682 ancillary file (2021-08-09)
Supplement: Supplementary file 1 [file 3-1.pdf]

## Retrosynthesis Route Preview

Compound Illustration: ■ Known ■ Novel

by qihan@accutarbio.com

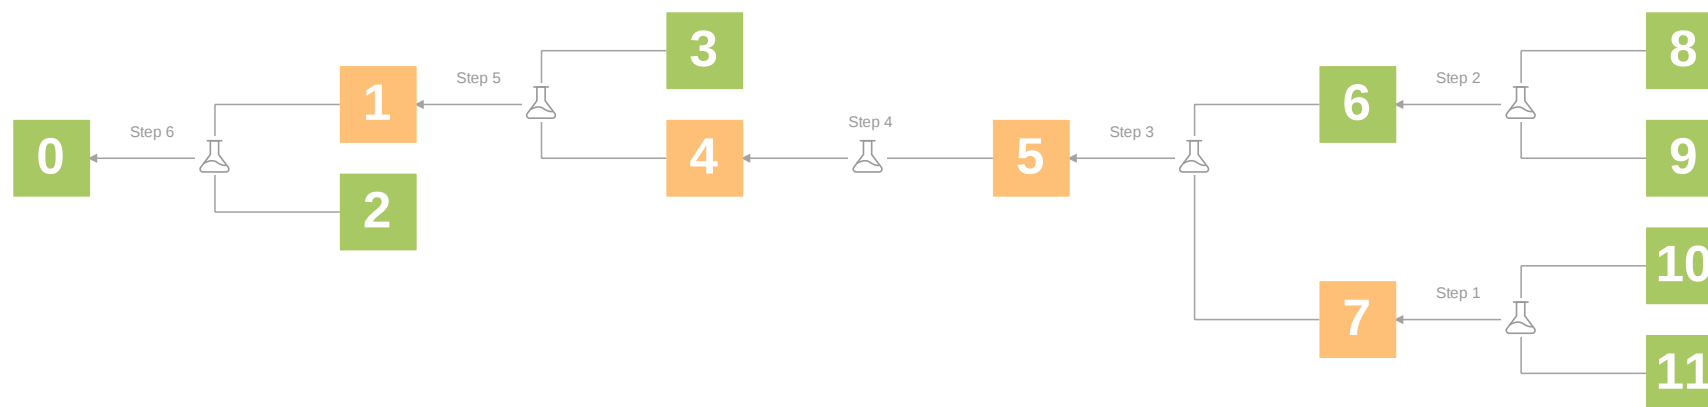

# Route Detail

Compound Illustration: ■ Known ■ Novel

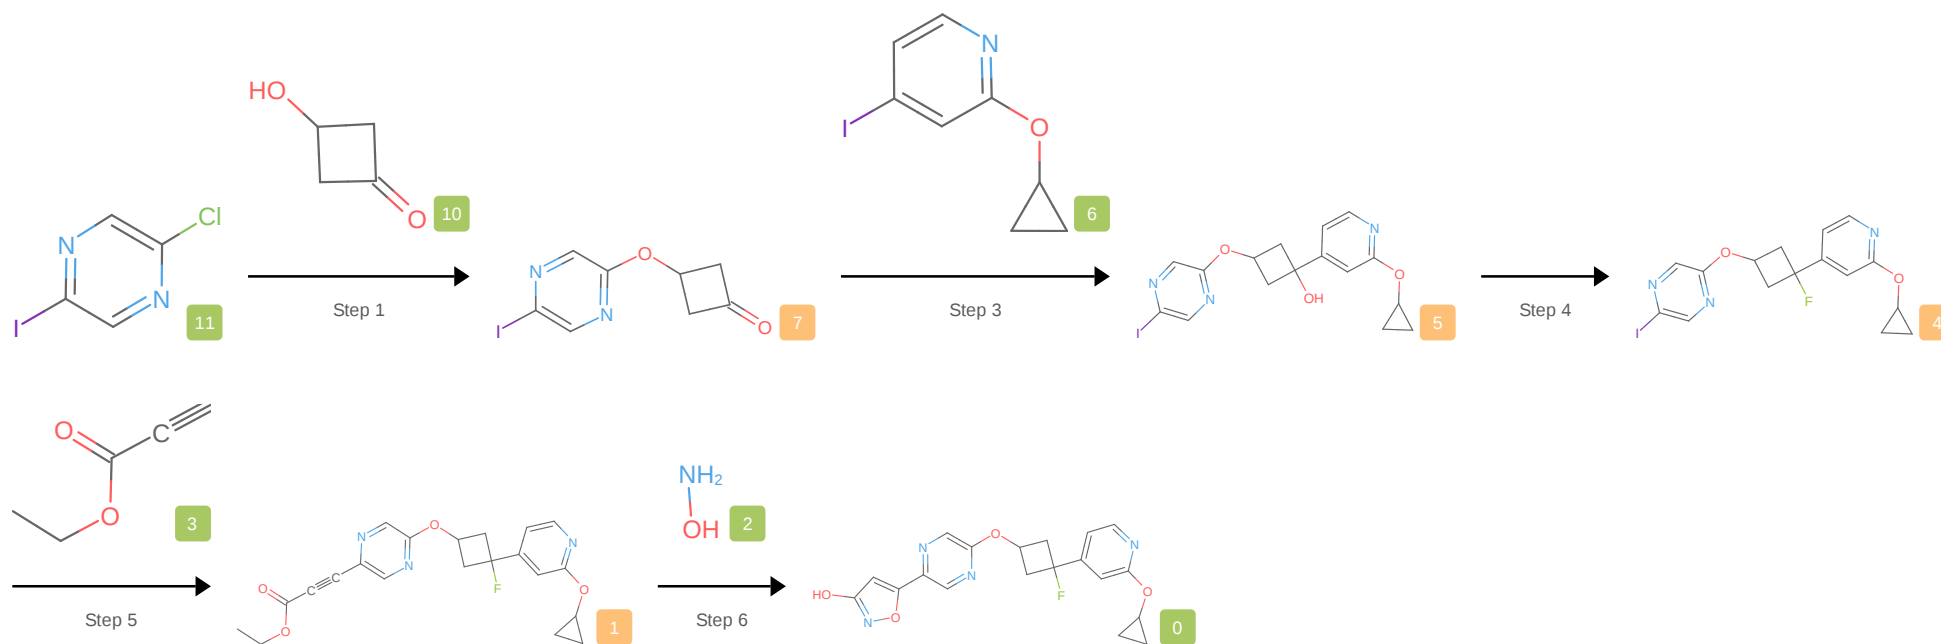

## Route Detail

Compound Illustration: ■ Known ■ Novel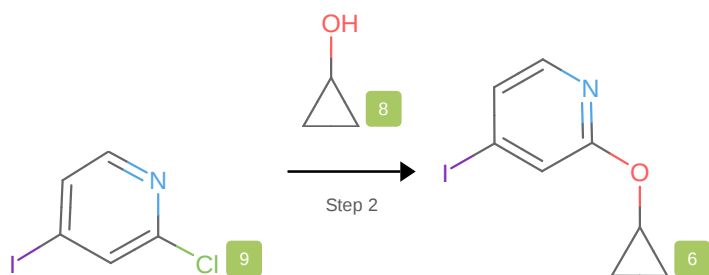

## Step Detail

Compound Illustration: ■ Known ■ Novel

### ◆ Step 1

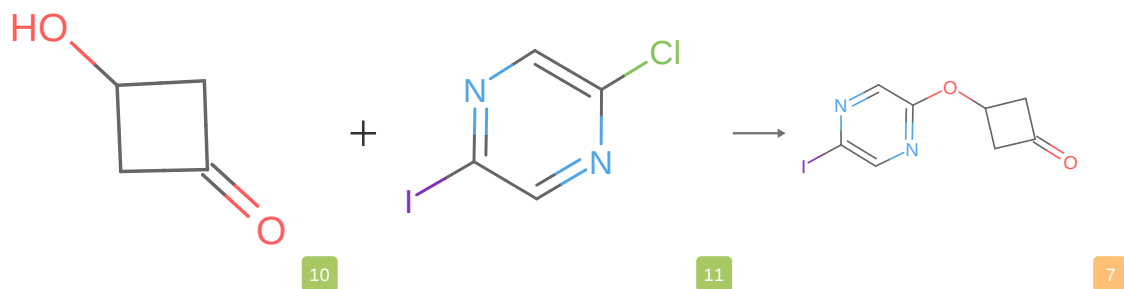

### ◆ Compound Detail

| Reactants Number | Molecular Formula                                | Molecular Weight | CAS Number                | PubChem CID           |
|------------------|--------------------------------------------------|------------------|---------------------------|-----------------------|
| 10               | C <sub>4</sub> H <sub>6</sub> O <sub>2</sub>     | 86.09 g/mol      | 15932-93-1    100058-61-5 | 22486676    153803888 |
| 11               | C <sub>4</sub> H <sub>2</sub> N <sub>2</sub> ClI | 240.43 g/mol     | 1057216-55-3              | 45789639              |

| Product Number | Molecular Formula                                             | Molecular Weight | CAS Number | PubChem CID |
|----------------|---------------------------------------------------------------|------------------|------------|-------------|
| 7              | C <sub>8</sub> H <sub>7</sub> N <sub>2</sub> O <sub>2</sub> I | 290.06 g/mol     |            |             |

### ◆ Reaction Condition

|           |                                              |
|-----------|----------------------------------------------|
| Condition | sodium hydroxide, 1-methyl-pyrrolidin-2-one. |
| Condition | sodium hydride, tetrahydrofuran.             |
| Condition | potassium tert-butyrate, tetrahydrofuran.    |

## Step Detail

Compound Illustration: ■ Known ■ Novel

### ◆ Step 2

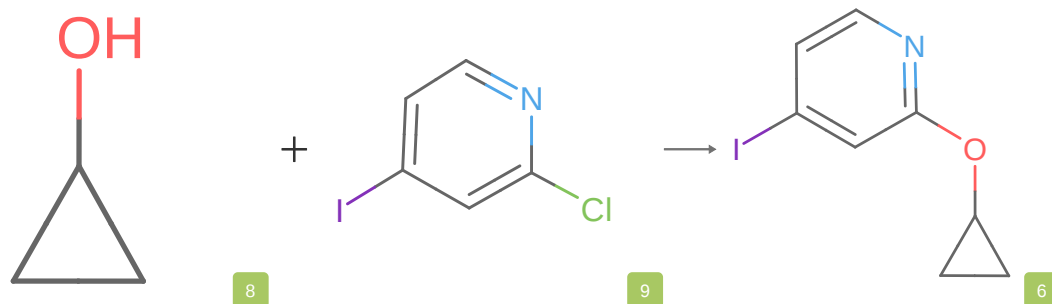

### ◆ Compound Detail

| Reactants Number | Molecular Formula                  | Molecular Weight | CAS Number |             |             | PubChem CID |          |          |
|------------------|------------------------------------|------------------|------------|-------------|-------------|-------------|----------|----------|
| 8                | C <sub>3</sub> H <sub>6</sub> O    | 58.08 g/mol      | 4606-06-8  | 5296-57-1   | 16545-68-9  | 123361      | 18457681 | 18764214 |
| 9                | C <sub>5</sub> H <sub>3</sub> NCII | 239.44 g/mol     | 78607-36-0 | 153034-86-7 | 168428-75-9 | 1516511     | 10105718 | 57941072 |

| Product Number | Molecular Formula                 | Molecular Weight | CAS Number   |  | PubChem CID |
|----------------|-----------------------------------|------------------|--------------|--|-------------|
| 6              | C <sub>8</sub> H <sub>8</sub> NOI | 261.06 g/mol     | 2090045-22-8 |  | 121231647   |

### ◆ Reaction Condition

|           |                                           |
|-----------|-------------------------------------------|
| Condition | sodium hydride.                           |
| Condition | sodium hydride, tetrahydrofuran.          |
| Condition | potassium tert-butyrate, tetrahydrofuran. |

## Step Detail

Compound Illustration: ■ Known ■ Novel

### ◆ Step 3

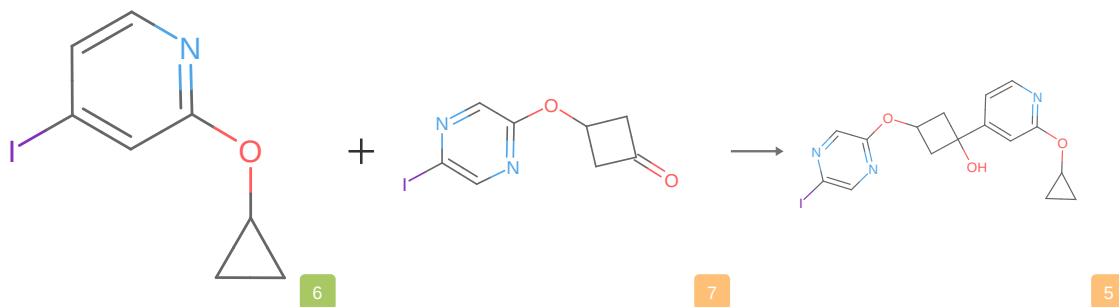

### ◆ Compound Detail

| Reactants Number | Molecular Formula                                             | Molecular Weight | CAS Number   | PubChem CID |
|------------------|---------------------------------------------------------------|------------------|--------------|-------------|
| 6                | C <sub>8</sub> H <sub>8</sub> NOI                             | 261.06 g/mol     | 2090045-22-8 | 121231647   |
| 7                | C <sub>8</sub> H <sub>7</sub> N <sub>2</sub> O <sub>2</sub> I | 290.06 g/mol     |              |             |

| Product Number | Molecular Formula                                               | Molecular Weight | CAS Number | PubChem CID |
|----------------|-----------------------------------------------------------------|------------------|------------|-------------|
| 5              | C <sub>16</sub> H <sub>16</sub> N <sub>3</sub> O <sub>3</sub> I | 425.22 g/mol     |            |             |

### ◆ Reaction Condition

|           |                                               |
|-----------|-----------------------------------------------|
| Condition | isopropylmagnesium chloride, tetrahydrofuran. |
| Condition | n-butyllithium, tetrahydrofuran.              |
| Condition | n-butyllithium.                               |

## Step Detail

Compound Illustration: ■ Known ■ Novel

### ◆ Step 4

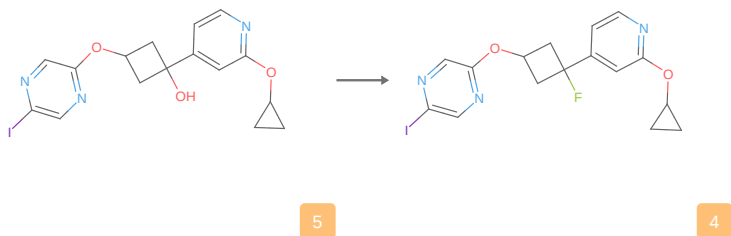

### ◆ Compound Detail

| Reactants Number | Molecular Formula                                               | Molecular Weight | CAS Number | PubChem CID |
|------------------|-----------------------------------------------------------------|------------------|------------|-------------|
| 5                | C <sub>16</sub> H <sub>16</sub> N <sub>3</sub> O <sub>3</sub> I | 425.22 g/mol     |            |             |

| Product Number | Molecular Formula                                                | Molecular Weight | CAS Number | PubChem CID |
|----------------|------------------------------------------------------------------|------------------|------------|-------------|
| 4              | C <sub>16</sub> H <sub>15</sub> N <sub>3</sub> O <sub>2</sub> FI | 427.21 g/mol     |            |             |

### ◆ Reaction Condition

|           |                                                                    |
|-----------|--------------------------------------------------------------------|
| Condition | diethylamino-sulfur trifluoride, dichloromethane.                  |
| Condition | diethylamino-sulfur trifluoride, dichloromethane, dichloromethane. |
| Condition | dichloromethane.                                                   |

## Step Detail

Compound Illustration: ■ Known ■ Novel

### ◆ Step 5

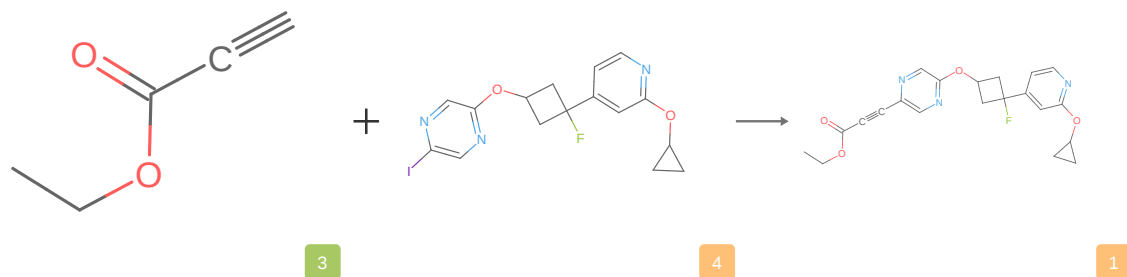

### ◆ Compound Detail

| Reactants Number | Molecular Formula                                                | Molecular Weight | CAS Number                         | PubChem CID                |
|------------------|------------------------------------------------------------------|------------------|------------------------------------|----------------------------|
| 3                | C <sub>5</sub> H <sub>6</sub> O <sub>2</sub>                     | 98.10 g/mol      | 623-47-2   59938-67-9   62500-21-4 | 12182   9837543   11029775 |
| 4                | C <sub>16</sub> H <sub>15</sub> N <sub>3</sub> O <sub>2</sub> FI | 427.21 g/mol     |                                    |                            |

| Product Number | Molecular Formula                                               | Molecular Weight | CAS Number | PubChem CID |
|----------------|-----------------------------------------------------------------|------------------|------------|-------------|
| 1              | C <sub>21</sub> H <sub>20</sub> N <sub>3</sub> O <sub>4</sub> F | 397.40 g/mol     |            |             |

### ◆ Reaction Condition

|           |                                                                                                    |
|-----------|----------------------------------------------------------------------------------------------------|
| Condition | copper(I) oxide, 1,4-dioxane.                                                                      |
| Condition | triethylamine, tetrakis(triphenylphosphine) palladium(0), tetrahydrofuran, N,N-dimethyl-formamide. |
| Condition | triethylamine, bis-triphenylphosphine-palladium(II) chloride, tetrahydrofuran.                     |



## Step Detail

Compound Illustration: ■ Known ■ Novel

### ◆ Step 6

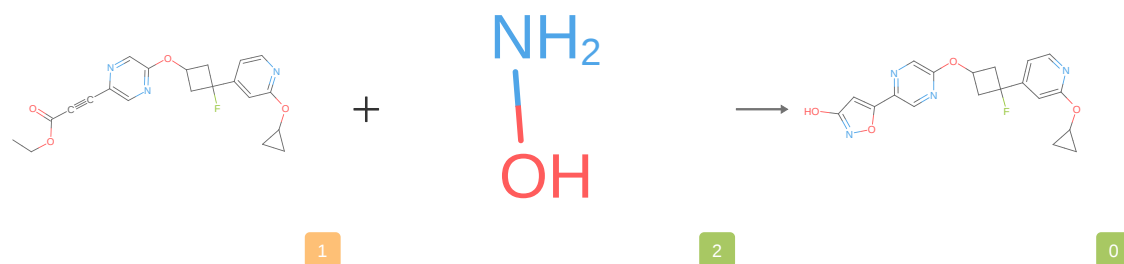

### ◆ Compound Detail

| Reactants Number | Molecular Formula                                               | Molecular Weight | CAS Number |           |           | PubChem CID |       |       |
|------------------|-----------------------------------------------------------------|------------------|------------|-----------|-----------|-------------|-------|-------|
| 1                | C <sub>21</sub> H <sub>20</sub> N <sub>3</sub> O <sub>4</sub> F | 397.40 g/mol     |            |           |           |             |       |       |
| 2                | H <sub>3</sub> NO                                               | 33.03 g/mol      | 5470-11-1  | 7232-25-9 | 7233-27-4 | 787         | 62160 | 64866 |

| Product Number | Molecular Formula                                               | Molecular Weight | CAS Number |  |  | PubChem CID |           |
|----------------|-----------------------------------------------------------------|------------------|------------|--|--|-------------|-----------|
| 0              | C <sub>19</sub> H <sub>17</sub> N <sub>4</sub> O <sub>4</sub> F | 384.37 g/mol     |            |  |  | 139450937   | 142378482 |

### ◆ Reaction Condition

|           |                                                                               |
|-----------|-------------------------------------------------------------------------------|
| Condition | water, sodium hydroxide, triethylamine, ethanol.                              |
| Condition | triethylamine, sodium hydroxide, HCl aq., ethanol, water, ethanol, ice water. |
| Condition | sodium hydroxide, hydrogenchloride, ethanol.                                  |
