# Supplementary material for: ChemiRise: a data-driven retrosynthesis engine
Source: arXiv:2108.04682 ancillary file (2021-08-09)
Supplement: Supplementary file 2 [file 3-2.pdf]

## Retrosynthesis Route Preview

Compound Illustration: ■ Known ■ Novel

by qihan@accutarbio.com

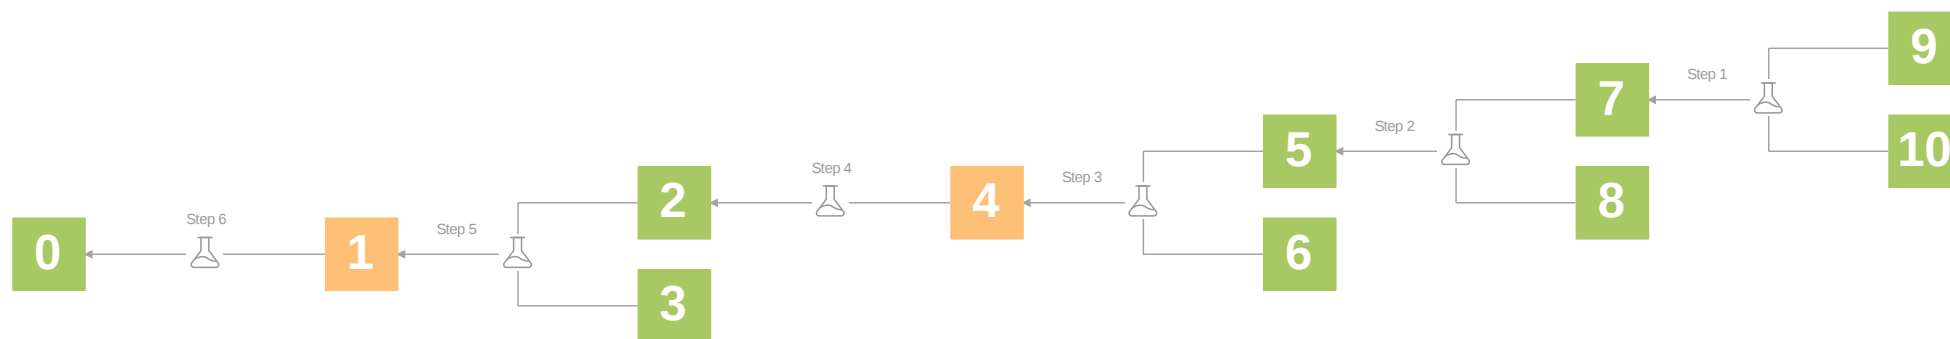

## Route Detail

Compound Illustration: ■ Known ■ Novel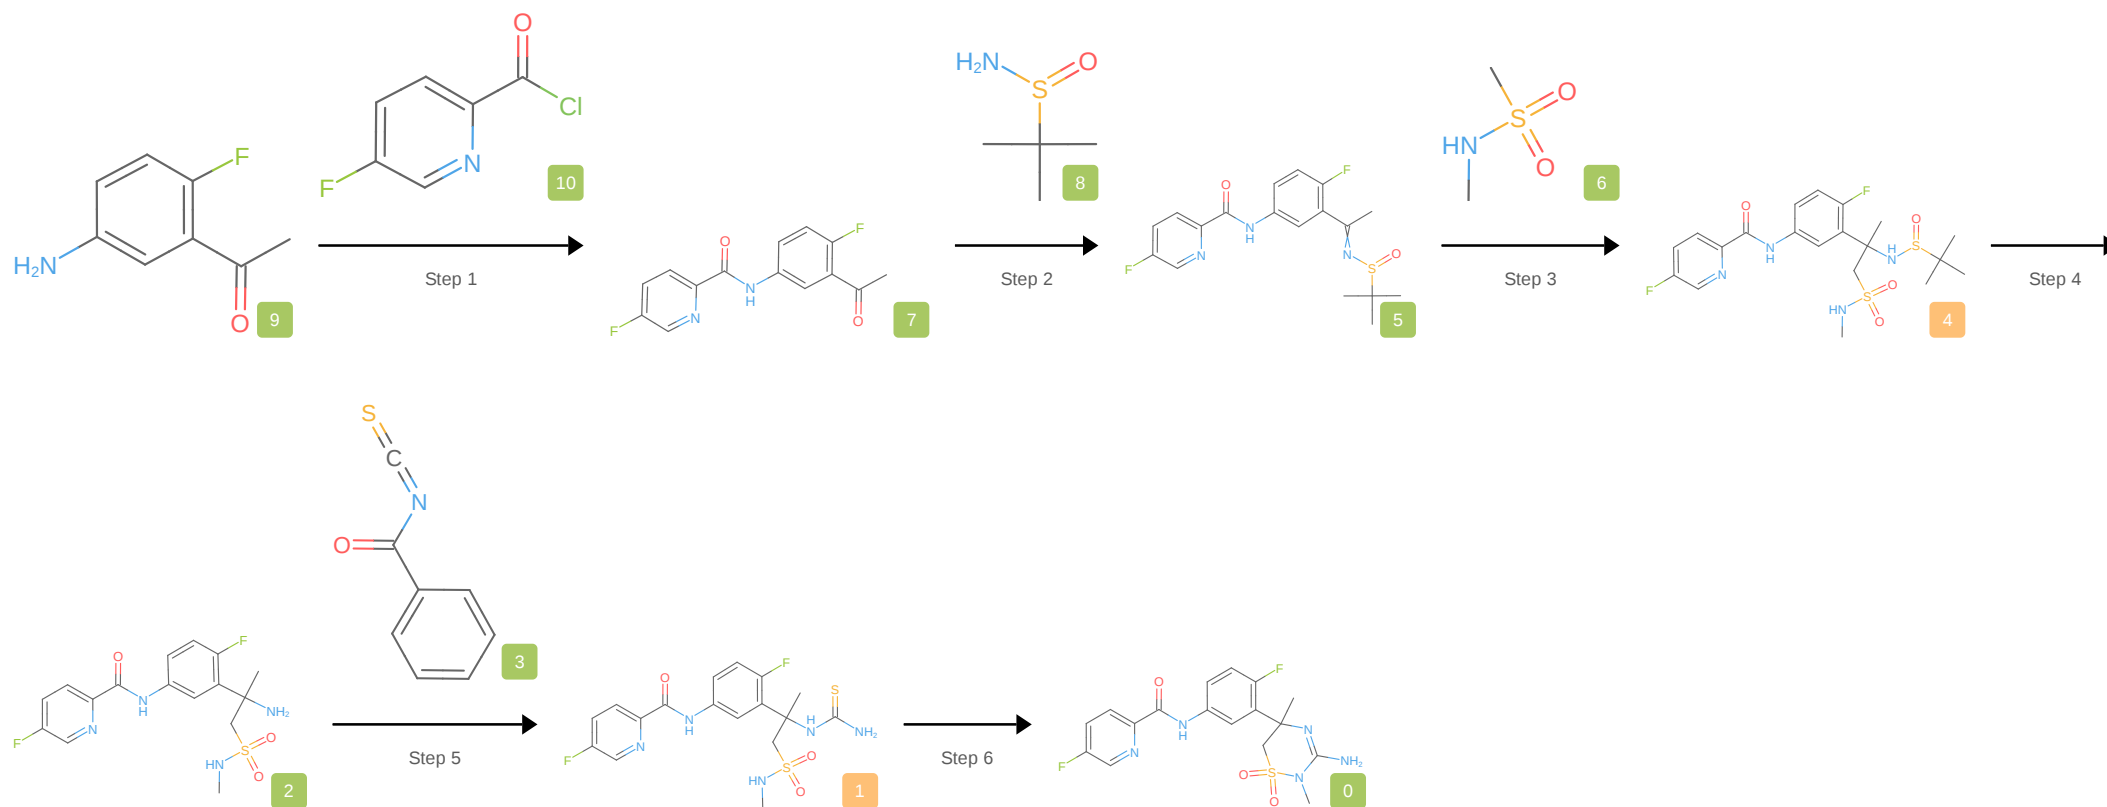

## Step Detail

Compound Illustration: ■ Known ■ Novel

### ◆ Step 1

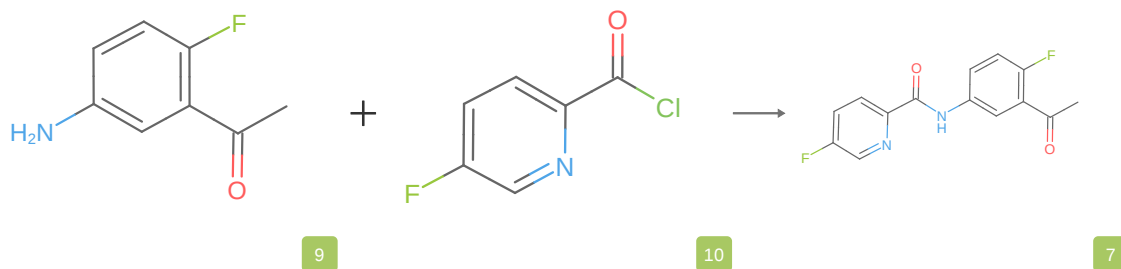

### ◆ Compound Detail

| Reactants Number | Molecular Formula                   | Molecular Weight | CAS Number                           | PubChem CID        |
|------------------|-------------------------------------|------------------|--------------------------------------|--------------------|
| 9                | C <sub>8</sub> H <sub>8</sub> NOF   | 153.16 g/mol     | 67500-19-0 1261838-05-4 1352568-63-8 | 2781125 71741807   |
| 10               | C <sub>6</sub> H <sub>3</sub> NOFCl | 159.55 g/mol     | 717871-83-5 2059971-46-7             | 21942698 137703077 |

| Product Number | Molecular Formula                                                            | Molecular Weight | CAS Number | PubChem CID |
|----------------|------------------------------------------------------------------------------|------------------|------------|-------------|
| 7              | C <sub>14</sub> H <sub>10</sub> N <sub>2</sub> O <sub>2</sub> F <sub>2</sub> | 276.24 g/mol     |            | 118864517   |

### ◆ Reaction Condition

|           |                                                |
|-----------|------------------------------------------------|
| Condition | N-ethyl-N,N-diisopropylamine, dichloromethane. |
| Condition | pyridine, dichloromethane.                     |
| Condition | triethylamine, tetrahydrofuran.                |

## Step Detail

Compound Illustration: ■ Known ■ Novel

### ◆ Step 2

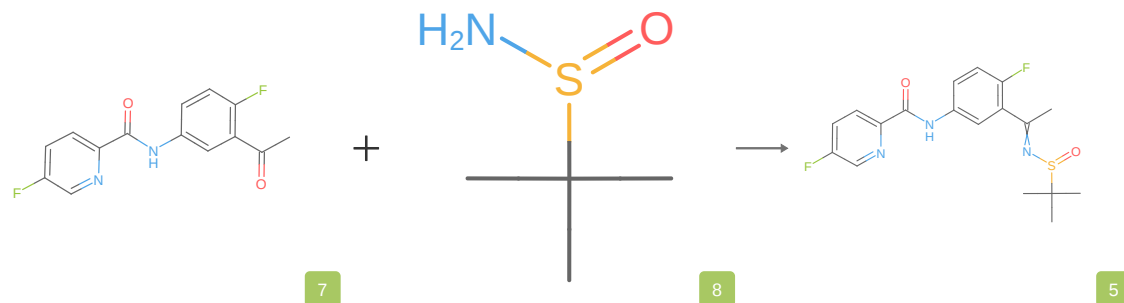

### ◆ Compound Detail

| Reactants Number | Molecular Formula                                                            | Molecular Weight | CAS Number                          | PubChem CID               |
|------------------|------------------------------------------------------------------------------|------------------|-------------------------------------|---------------------------|
| 7                | C <sub>14</sub> H <sub>10</sub> N <sub>2</sub> O <sub>2</sub> F <sub>2</sub> | 276.24 g/mol     |                                     | 118864517                 |
| 8                | C <sub>4</sub> H <sub>11</sub> NOS                                           | 121.20 g/mol     | 146374-27-8 196929-78-9 343338-28-3 | 3382465 57658914 58516118 |

| Product Number | Molecular Formula                                                              | Molecular Weight | CAS Number | PubChem CID         |
|----------------|--------------------------------------------------------------------------------|------------------|------------|---------------------|
| 5              | C <sub>18</sub> H <sub>19</sub> N <sub>3</sub> O <sub>2</sub> F <sub>2</sub> S | 379.43 g/mol     |            | 118883407 130331611 |

### ◆ Reaction Condition

|           |                                                |
|-----------|------------------------------------------------|
| Condition | titanium(IV) tetraethanolate, tetrahydrofuran. |
| Condition | ethanol.                                       |
| Condition | acetic acid, ethanol.                          |

## Step Detail

Compound Illustration: ■ Known ■ Novel

### ◆ Step 3

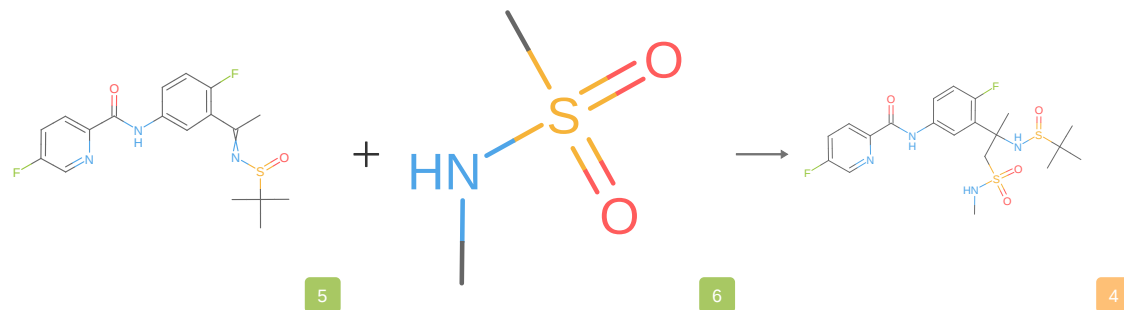

### ◆ Compound Detail

| Reactants Number | Molecular Formula                                                              | Molecular Weight | CAS Number | PubChem CID             |
|------------------|--------------------------------------------------------------------------------|------------------|------------|-------------------------|
| 5                | C <sub>18</sub> H <sub>19</sub> N <sub>3</sub> O <sub>2</sub> F <sub>2</sub> S | 379.43 g/mol     |            | 118883407 130331611     |
| 6                | C <sub>2</sub> H <sub>7</sub> NO <sub>2</sub> S                                | 109.15 g/mol     | 1184-85-6  | 97632 12738561 18345640 |

| Product Number | Molecular Formula                                                                           | Molecular Weight | CAS Number | PubChem CID |
|----------------|---------------------------------------------------------------------------------------------|------------------|------------|-------------|
| 4              | C <sub>20</sub> H <sub>26</sub> N <sub>4</sub> O <sub>4</sub> F <sub>2</sub> S <sub>2</sub> | 488.58 g/mol     |            |             |

### ◆ Reaction Condition

|           |                                                     |
|-----------|-----------------------------------------------------|
| Condition | n-butyllithium, tetrahydrofuran, hexane.            |
| Condition | n-butyllithium.                                     |
| Condition | lithium diisopropyl amide, tetrahydrofuran, hexane. |

## Step Detail

Compound Illustration: ■ Known ■ Novel

### ◆ Step 4

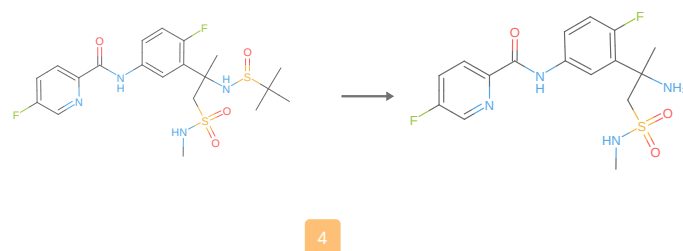

### ◆ Compound Detail

| Reactants Number | Molecular Formula                                                                           | Molecular Weight | CAS Number | PubChem CID |
|------------------|---------------------------------------------------------------------------------------------|------------------|------------|-------------|
| 4                | C <sub>20</sub> H <sub>26</sub> N <sub>4</sub> O <sub>4</sub> F <sub>2</sub> S <sub>2</sub> | 488.58 g/mol     |            |             |

| Product Number | Molecular Formula                                                              | Molecular Weight | CAS Number | PubChem CID |
|----------------|--------------------------------------------------------------------------------|------------------|------------|-------------|
| 2              | C <sub>16</sub> H <sub>18</sub> N <sub>4</sub> O <sub>3</sub> F <sub>2</sub> S | 384.40 g/mol     |            | 118864500   |

### ◆ Reaction Condition

|           |                                          |
|-----------|------------------------------------------|
| Condition | hydrogenchloride, 1,4-dioxane.           |
| Condition | hydrogenchloride, 1,4-dioxane, methanol. |
| Condition | hydrogenchloride.                        |

## Step Detail

Compound Illustration: ■ Known ■ Novel

### ◆ Step 5

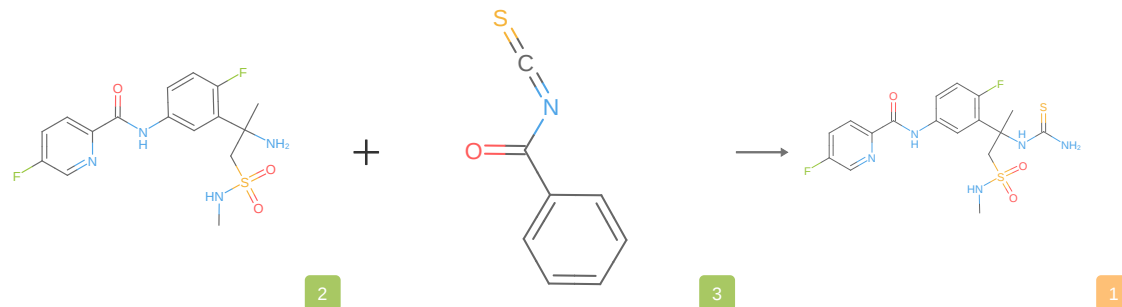

### ◆ Compound Detail

| Reactants Number | Molecular Formula                                                              | Molecular Weight | CAS Number | PubChem CID             |
|------------------|--------------------------------------------------------------------------------|------------------|------------|-------------------------|
| 2                | C <sub>16</sub> H <sub>18</sub> N <sub>4</sub> O <sub>3</sub> F <sub>2</sub> S | 384.40 g/mol     |            | 118864500               |
| 3                | C <sub>8</sub> H <sub>5</sub> NOS                                              | 163.20 g/mol     | 532-55-8   | 68284 20547025 58638775 |

| Product Number | Molecular Formula                                                                           | Molecular Weight | CAS Number | PubChem CID |
|----------------|---------------------------------------------------------------------------------------------|------------------|------------|-------------|
| 1              | C <sub>17</sub> H <sub>19</sub> N <sub>5</sub> O <sub>3</sub> F <sub>2</sub> S <sub>2</sub> | 443.50 g/mol     |            |             |

### ◆ Reaction Condition

|           |                                                |
|-----------|------------------------------------------------|
| Condition | N-ethyl-N,N-diisopropylamine, dichloromethane. |
| Condition | sodium methylate, dichloromethane, methanol.   |
| Condition | ammonia, methanol.                             |

## Step Detail

Compound Illustration: ■ Known ■ Novel

### ◆ Step 6

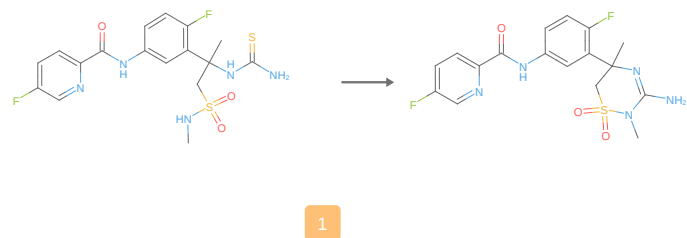

### ◆ Compound Detail

| Reactants Number | Molecular Formula                                                                           | Molecular Weight | CAS Number | PubChem CID |
|------------------|---------------------------------------------------------------------------------------------|------------------|------------|-------------|
| 1                | C <sub>17</sub> H <sub>19</sub> N <sub>5</sub> O <sub>3</sub> F <sub>2</sub> S <sub>2</sub> | 443.50 g/mol     |            |             |

| Product Number | Molecular Formula                                                              | Molecular Weight | CAS Number                   | PubChem CID |
|----------------|--------------------------------------------------------------------------------|------------------|------------------------------|-------------|
| 0              | C <sub>17</sub> H <sub>17</sub> N <sub>5</sub> O <sub>3</sub> F <sub>2</sub> S | 409.41 g/mol     | 1286770-55-5    2095432-65-6 | 75629988    |

### ◆ Reaction Condition

| Condition | methyl iodide.                               |
|-----------|----------------------------------------------|
| Condition | N-ethyl-N,N-diisopropylamine, methyl iodide. |
