# Supplementary material for: ChemiRise: a data-driven retrosynthesis engine
Source: arXiv:2108.04682 ancillary file (2021-08-09)
Supplement: Supplementary file 3 [file 3-3.pdf]

## Retrosynthesis Route Preview

Compound Illustration: ■ Known ■ Novel

by qihan@accutarbio.com

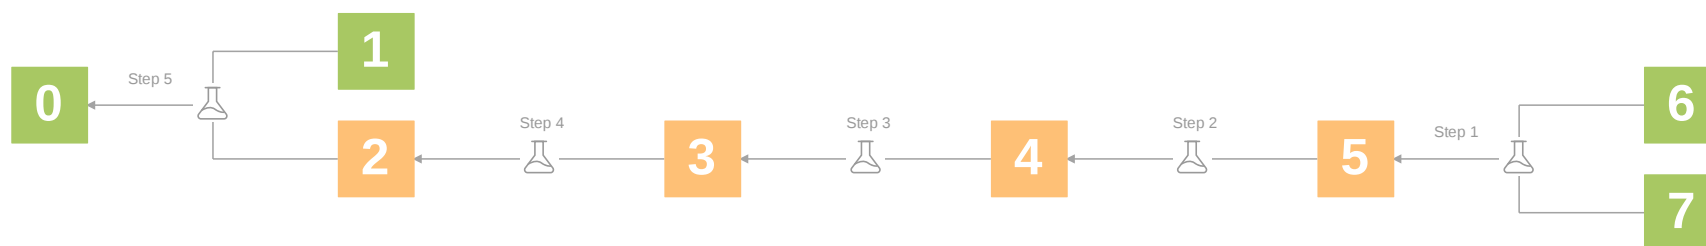

## Route Detail

Compound Illustration: ■ Known ■ Novel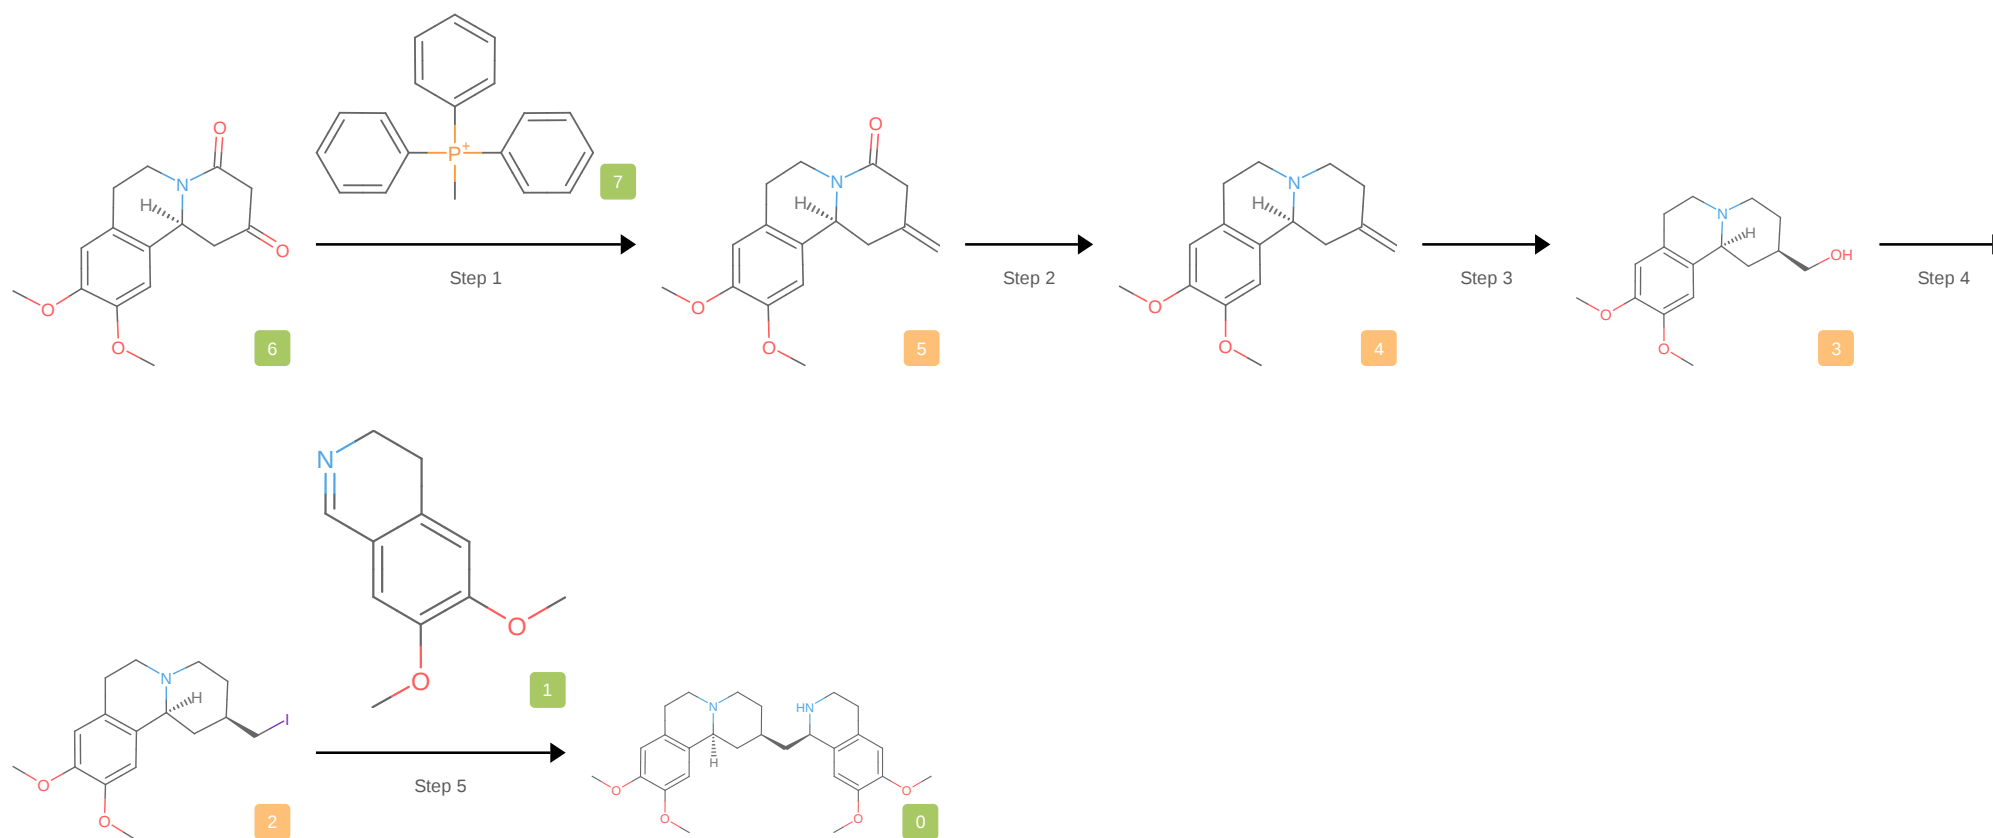

## Step Detail

Compound Illustration: ■ Known ■ Novel

### ◆ Step 1

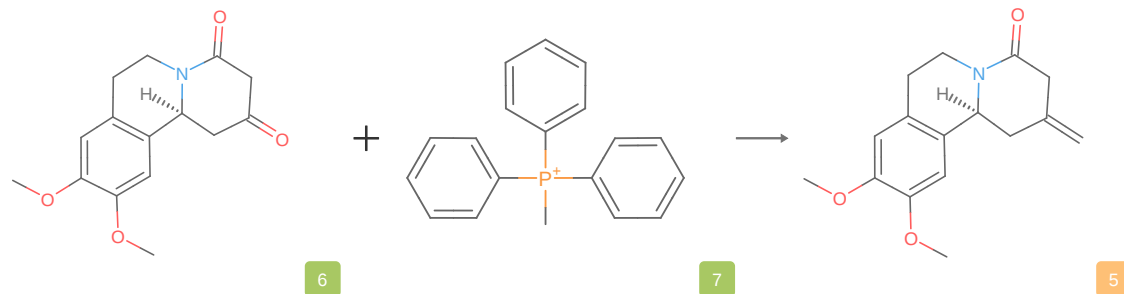

### ◆ Compound Detail

| Reactants Number | Molecular Formula                               | Molecular Weight | CAS Number |           |           | PubChem CID |         |        |
|------------------|-------------------------------------------------|------------------|------------|-----------|-----------|-------------|---------|--------|
| 6                | C <sub>15</sub> H <sub>17</sub> NO <sub>4</sub> | 275.30 g/mol     | 5911-65-9  |           |           | 7096092     | 3379225 |        |
| 7                | C <sub>19</sub> H <sub>18</sub> P               | 277.33 g/mol     | 1031-15-8  | 1560-52-7 | 1560-56-1 | 74505       | 74506   | 638159 |

| Product Number | Molecular Formula                               | Molecular Weight | CAS Number |  |  | PubChem CID |  |  |
|----------------|-------------------------------------------------|------------------|------------|--|--|-------------|--|--|
| 5              | C <sub>16</sub> H <sub>19</sub> NO <sub>3</sub> | 273.33 g/mol     |            |  |  |             |  |  |

### ◆ Reaction Condition

|           |                                                             |
|-----------|-------------------------------------------------------------|
| Condition | n-butyllithium, tetrahydrofuran, hexane, hydrogen bromide.  |
| Condition | potassium tert-butyrate, tetrahydrofuran, hydrogen bromide. |
| Condition | n-butyllithium, hydrogen bromide.                           |

## Step Detail

Compound Illustration: ■ Known ■ Novel

### ◆ Step 2

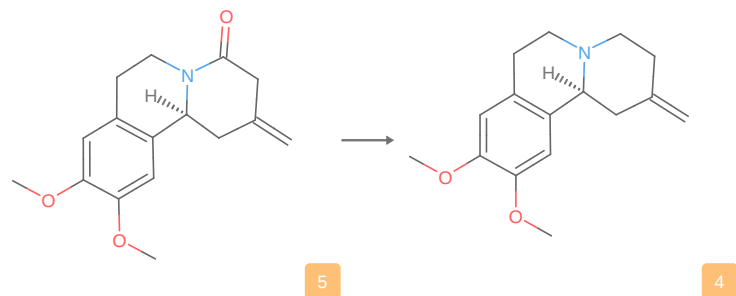

### ◆ Compound Detail

| Reactants Number | Molecular Formula                               | Molecular Weight | CAS Number | PubChem CID |
|------------------|-------------------------------------------------|------------------|------------|-------------|
| 5                | C <sub>16</sub> H <sub>19</sub> NO <sub>3</sub> | 273.33 g/mol     |            |             |

| Product Number | Molecular Formula                               | Molecular Weight | CAS Number | PubChem CID |
|----------------|-------------------------------------------------|------------------|------------|-------------|
| 4              | C <sub>16</sub> H <sub>21</sub> NO <sub>2</sub> | 259.35 g/mol     |            |             |

### ◆ Reaction Condition

|           |                                                  |
|-----------|--------------------------------------------------|
| Condition | borane-THF, tetrahydrofuran.                     |
| Condition | lithium aluminium tetrahydride, tetrahydrofuran. |
| Condition | lithium aluminium tetrahydride.                  |

## Step Detail

Compound Illustration: ■ Known ■ Novel

### ◆ Step 3

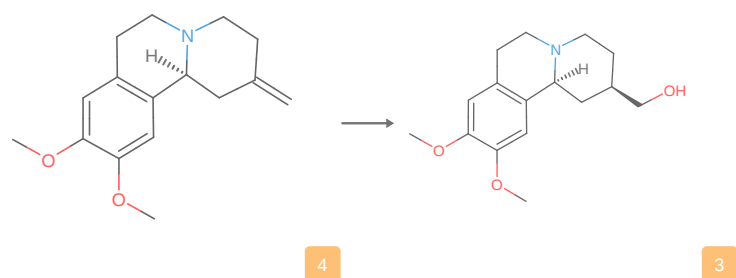

### ◆ Compound Detail

| Reactants Number | Molecular Formula                               | Molecular Weight | CAS Number | PubChem CID |
|------------------|-------------------------------------------------|------------------|------------|-------------|
| 4                | C <sub>16</sub> H <sub>21</sub> NO <sub>2</sub> | 259.35 g/mol     |            |             |

| Product Number | Molecular Formula                               | Molecular Weight | CAS Number | PubChem CID |
|----------------|-------------------------------------------------|------------------|------------|-------------|
| 3              | C <sub>16</sub> H <sub>23</sub> NO <sub>3</sub> | 277.36 g/mol     |            |             |

### ◆ Reaction Condition

|           |                                                                                      |
|-----------|--------------------------------------------------------------------------------------|
| Condition | borane-THF, dihydrogen peroxide, sodium hydroxide, tetrahydrofuran.                  |
| Condition | 9-bora-bicyclo[3.3.1]nonane, dihydrogen peroxide, sodium hydroxide, tetrahydrofuran. |
| Condition | sodium hydroxide, 9-borabicyclo[3.3.1]nonane dimer, dihydrogen peroxide.             |

## Step Detail

Compound Illustration: ■ Known ■ Novel

## ◆ Step 4

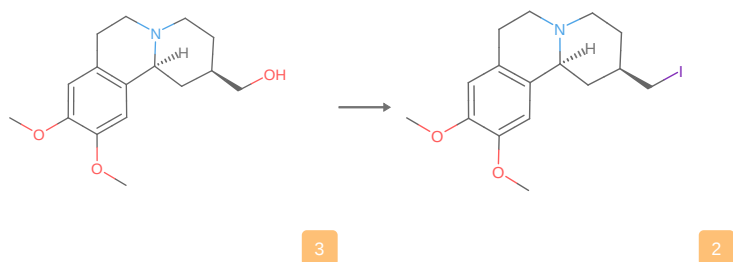

## ◆ Compound Detail

| Reactants Number | Molecular Formula                               | Molecular Weight | CAS Number | PubChem CID |
|------------------|-------------------------------------------------|------------------|------------|-------------|
| 3                | C <sub>16</sub> H <sub>23</sub> NO <sub>3</sub> | 277.36 g/mol     |            |             |

| Product Number | Molecular Formula                                 | Molecular Weight | CAS Number | PubChem CID |
|----------------|---------------------------------------------------|------------------|------------|-------------|
| 2              | C <sub>16</sub> H <sub>22</sub> NO <sub>2</sub> I | 387.25 g/mol     |            |             |

## ◆ Reaction Condition

|           |                                                                |
|-----------|----------------------------------------------------------------|
| Condition | 1H-imidazole, triphenylphosphine, benzene.                     |
| Condition | 1H-imidazole, triphenylphosphine, diethyl ether, acetonitrile. |
| Condition | 1H-imidazole, triphenylphosphine, toluene.                     |

## Step Detail

Compound Illustration: ■ Known ■ Novel

### ◆ Step 5

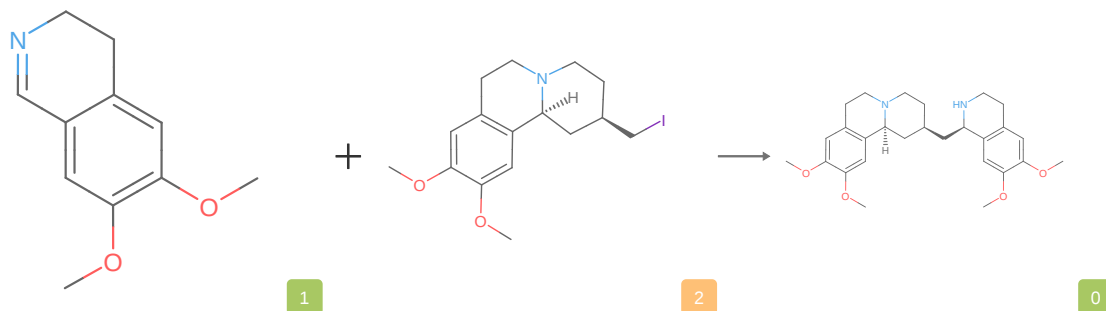

### ◆ Compound Detail

| Reactants Number | Molecular Formula                                 | Molecular Weight | CAS Number                       | PubChem CID        |
|------------------|---------------------------------------------------|------------------|----------------------------------|--------------------|
| 1                | C <sub>11</sub> H <sub>13</sub> NO <sub>2</sub>   | 191.23 g/mol     | 3382-18-1 20232-39-7 133348-02-4 | 30057 30058 487617 |
| 2                | C <sub>16</sub> H <sub>22</sub> NO <sub>2</sub> I | 387.25 g/mol     |                                  |                    |

| Product Number | Molecular Formula                                             | Molecular Weight | CAS Number | PubChem CID |
|----------------|---------------------------------------------------------------|------------------|------------|-------------|
| 0              | C <sub>27</sub> H <sub>36</sub> N <sub>2</sub> O <sub>4</sub> | 452.59 g/mol     |            | 138551092   |

### ◆ Reaction Condition

|           |                                            |
|-----------|--------------------------------------------|
| Condition | indium, silver(I) iodide, water.           |
| Condition | strontium, tetrahydrofuran.                |
| Condition | indium, silver(I) iodide, methanol, water. |
