# Supplementary material for: ChemiRise: a data-driven retrosynthesis engine
Source: arXiv:2108.04682 ancillary file (2021-08-09)
Supplement: Supplementary file 4 [file 3-4.pdf]

## Retrosynthesis Route Preview

Compound Illustration: ■ Known ■ Novel

by qihan@accutarbio.com

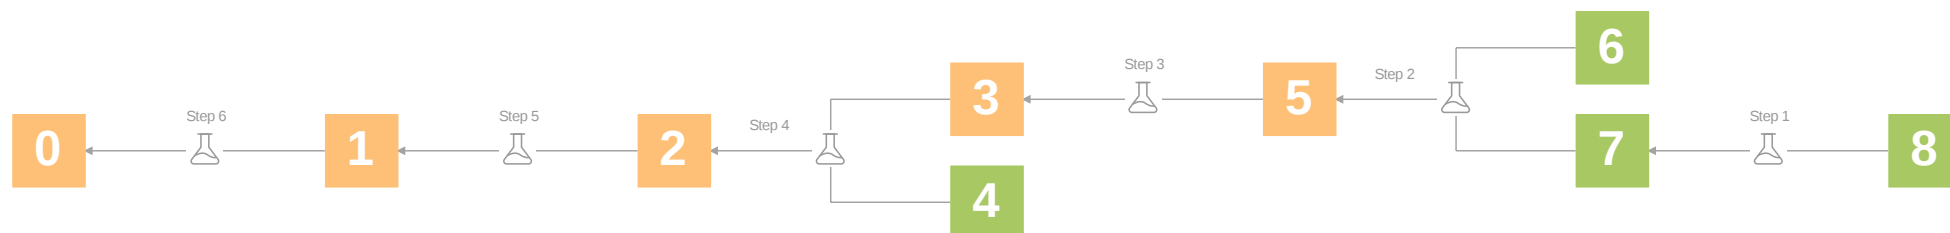

# Route Detail

Compound Illustration: ■ Known ■ Novel

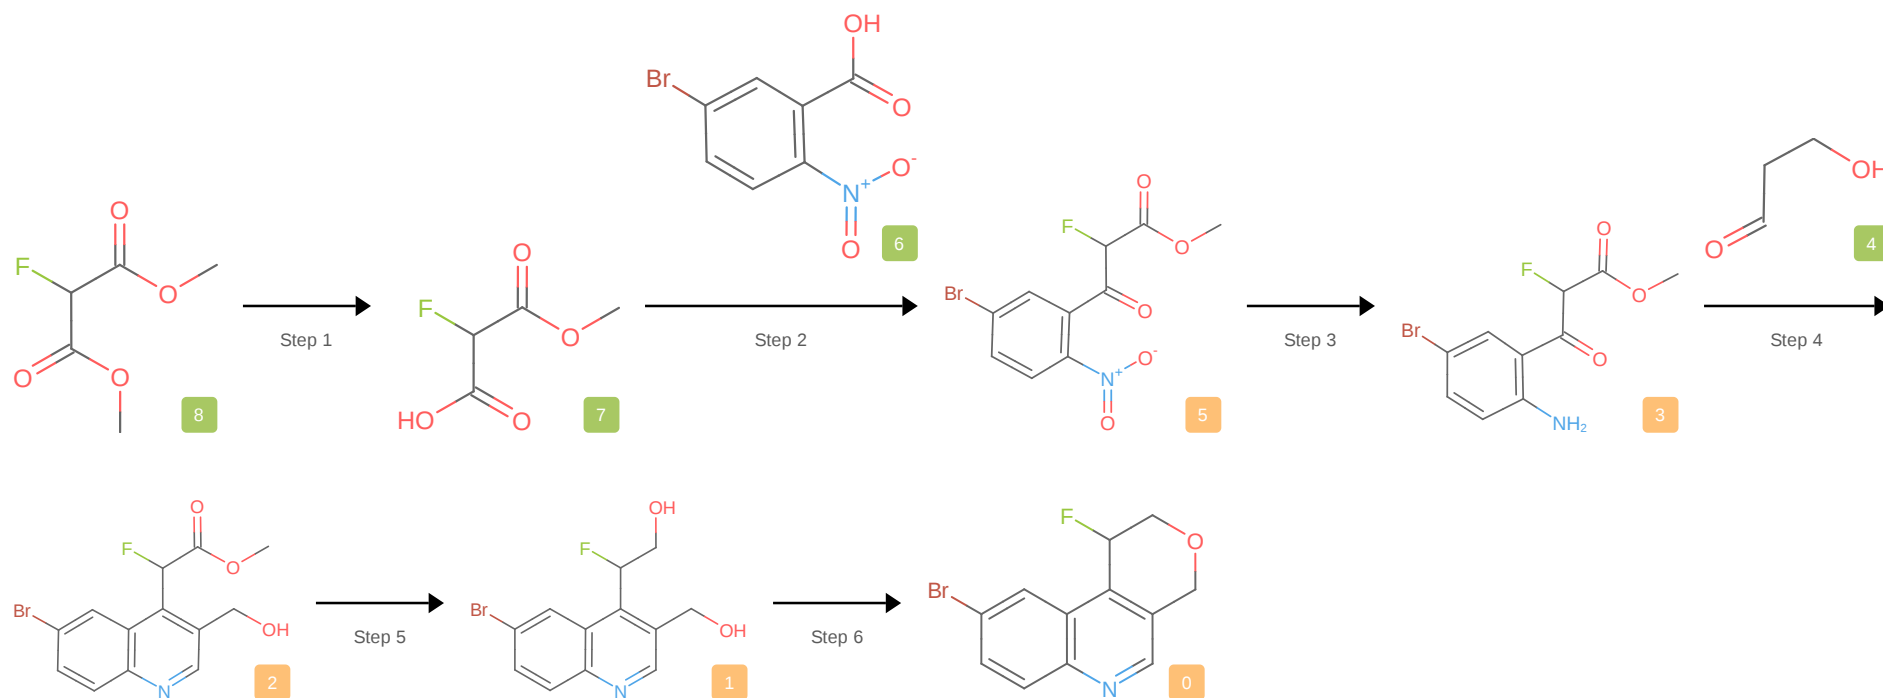

## Step Detail

Compound Illustration: ■ Known ■ Novel

### ◆ Step 1

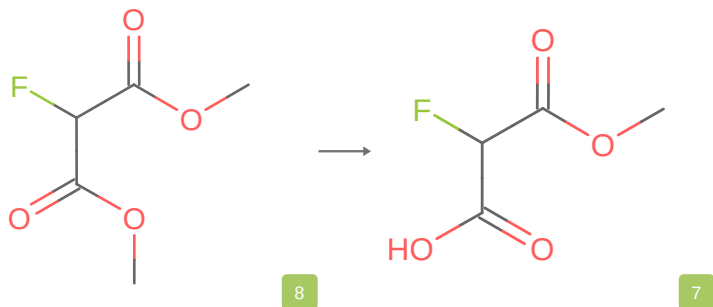

### ◆ Compound Detail

| Reactants Number | Molecular Formula                              | Molecular Weight | CAS Number | PubChem CID |
|------------------|------------------------------------------------|------------------|------------|-------------|
| 8                | C <sub>5</sub> H <sub>7</sub> O <sub>4</sub> F | 150.10 g/mol     | 344-14-9   | 2737111     |

| Product Number | Molecular Formula                              | Molecular Weight | CAS Number  | PubChem CID        |
|----------------|------------------------------------------------|------------------|-------------|--------------------|
| 7              | C <sub>4</sub> H <sub>5</sub> O <sub>4</sub> F | 136.08 g/mol     | 139590-63-9 | 15176477 131742526 |

### ◆ Reaction Condition

| Condition | lithium hydroxide, tetrahydrofuran.           |
|-----------|-----------------------------------------------|
| Condition | lithium hydroxide, tetrahydrofuran, methanol. |
| Condition | sodium hydroxide, methanol.                   |

## Step Detail

Compound Illustration: ■ Known ■ Novel

### ◆ Step 2

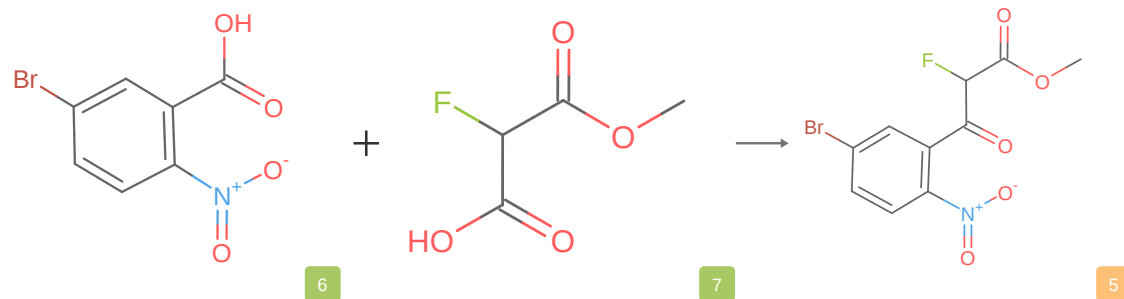

### ◆ Compound Detail

| Reactants Number | Molecular Formula                                | Molecular Weight | CAS Number  | PubChem CID |           |
|------------------|--------------------------------------------------|------------------|-------------|-------------|-----------|
| 6                | C <sub>7</sub> H <sub>4</sub> NO <sub>4</sub> Br | 246.02 g/mol     | 6950-43-2   | 248528      | 36690439  |
| 7                | C <sub>4</sub> H <sub>5</sub> O <sub>4</sub> F   | 136.08 g/mol     | 139590-63-9 | 15176477    | 131742526 |

| Product Number | Molecular Formula                                  | Molecular Weight | CAS Number | PubChem CID |  |
|----------------|----------------------------------------------------|------------------|------------|-------------|--|
| 5              | C <sub>10</sub> H <sub>7</sub> NO <sub>5</sub> FBr | 320.07 g/mol     |            |             |  |

### ◆ Reaction Condition

|           |                                                                                                                         |
|-----------|-------------------------------------------------------------------------------------------------------------------------|
| Condition | 1,1'-carbonyldiimidazole, tetrahydrofuran, magnesium.                                                                   |
| Condition | 1,1'-carbonyldiimidazole, magnesium chloride, tetrahydrofuran, potassium hydride.                                       |
| Condition | diethyl cyanophosphonate, benzotriazol-1-ol, triethylamine, trifluoroacetic acid, Wang resin, diisopropyl-carbodiimide. |

## Step Detail

Compound Illustration: ■ Known ■ Novel

### ◆ Step 3

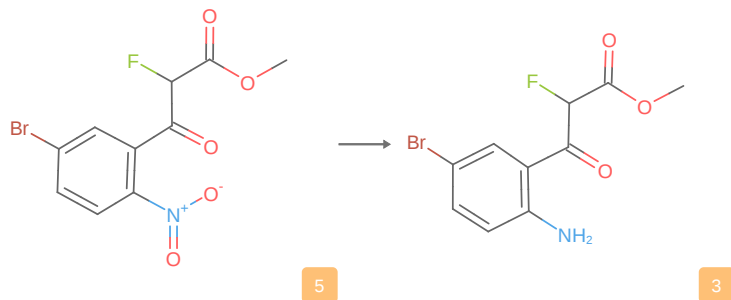

### ◆ Compound Detail

| Reactants Number | Molecular Formula                                  | Molecular Weight | CAS Number | PubChem CID |
|------------------|----------------------------------------------------|------------------|------------|-------------|
| 5                | C <sub>10</sub> H <sub>7</sub> NO <sub>5</sub> FBr | 320.07 g/mol     |            |             |

| Product Number | Molecular Formula                                  | Molecular Weight | CAS Number | PubChem CID |
|----------------|----------------------------------------------------|------------------|------------|-------------|
| 3              | C <sub>10</sub> H <sub>9</sub> NO <sub>3</sub> FBr | 290.09 g/mol     |            |             |

### ◆ Reaction Condition

|           |                                          |
|-----------|------------------------------------------|
| Condition | iron, ammonium chloride, ethanol, water. |
| Condition | ethyl acetate.                           |
| Condition | iron, acetic acid.                       |

## Step Detail

Compound Illustration: ■ Known ■ Novel

### ◆ Step 4

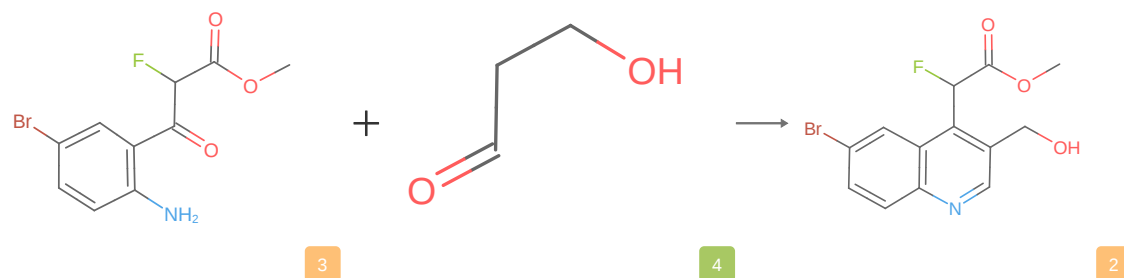

### ◆ Compound Detail

| Reactants Number | Molecular Formula                                  | Molecular Weight | CAS Number |            |            | PubChem CID |          |          |
|------------------|----------------------------------------------------|------------------|------------|------------|------------|-------------|----------|----------|
| 3                | C <sub>10</sub> H <sub>9</sub> NO <sub>3</sub> FBr | 290.09 g/mol     |            |            |            |             |          |          |
| 4                | C <sub>3</sub> H <sub>6</sub> O <sub>2</sub>       | 74.08 g/mol      | 2134-29-4  | 52030-92-9 | 75949-79-0 | 75049       | 10313159 | 10313160 |

| Product Number | Molecular Formula                                   | Molecular Weight | CAS Number |  |  | PubChem CID |  |  |
|----------------|-----------------------------------------------------|------------------|------------|--|--|-------------|--|--|
| 2              | C <sub>13</sub> H <sub>11</sub> NO <sub>3</sub> FBr | 328.14 g/mol     |            |  |  |             |  |  |

### ◆ Reaction Condition

|           |                                                                                 |
|-----------|---------------------------------------------------------------------------------|
| Condition | sulfuric acid, acetic acid.                                                     |
| Condition | 2,4,6-tripropyl-1,3,5,2,4,6-trioxatriphosphinane-2,4,6-trioxide, ethyl acetate. |
| Condition | potassium hydroxide, ethanol.                                                   |

## Step Detail

Compound Illustration: ■ Known ■ Novel

### ◆ Step 5

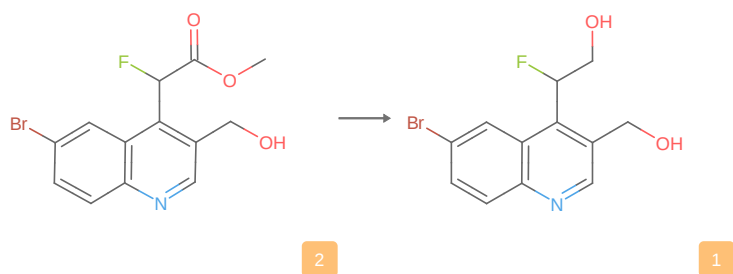

### ◆ Compound Detail

| Reactants Number | Molecular Formula                                   | Molecular Weight | CAS Number | PubChem CID |
|------------------|-----------------------------------------------------|------------------|------------|-------------|
| 2                | C <sub>13</sub> H <sub>11</sub> NO <sub>3</sub> FBr | 328.14 g/mol     |            |             |

| Product Number | Molecular Formula                                   | Molecular Weight | CAS Number | PubChem CID |
|----------------|-----------------------------------------------------|------------------|------------|-------------|
| 1              | C <sub>12</sub> H <sub>11</sub> NO <sub>2</sub> FBr | 300.13 g/mol     |            |             |

### ◆ Reaction Condition

|           |                                       |
|-----------|---------------------------------------|
| Condition | sodium tetrahydroborate, methanol.    |
| Condition | lithium aluminium tetrahydride.       |
| Condition | lithium borohydride, tetrahydrofuran. |

## Step Detail

Compound Illustration: ■ Known ■ Novel

### ◆ Step 6

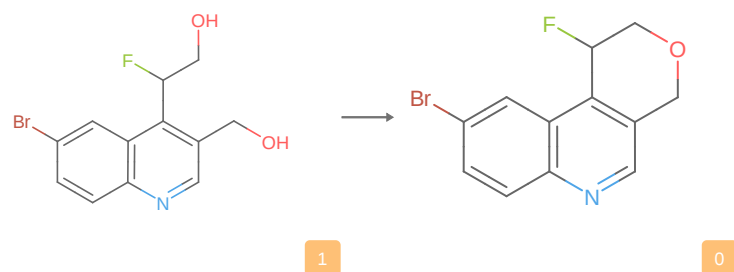

### ◆ Compound Detail

| Reactants Number | Molecular Formula                                   | Molecular Weight | CAS Number | PubChem CID |
|------------------|-----------------------------------------------------|------------------|------------|-------------|
| 1                | C <sub>12</sub> H <sub>11</sub> NO <sub>2</sub> FBr | 300.13 g/mol     |            |             |

| Product Number | Molecular Formula                    | Molecular Weight | CAS Number | PubChem CID |
|----------------|--------------------------------------|------------------|------------|-------------|
| 0              | C <sub>12</sub> H <sub>9</sub> NOFBr | 282.11 g/mol     |            |             |

### ◆ Reaction Condition

|           |                                                       |
|-----------|-------------------------------------------------------|
| Condition | acetonitrile.                                         |
| Condition | triphenylphosphine, diethylazodicarboxylate, toluene. |
| Condition | trifluoroacetic acid, 1,2-dichloro-ethane.            |
