# Supplementary material for: ChemiRise: a data-driven retrosynthesis engine
Source: arXiv:2108.04682 ancillary file (2021-08-09)
Supplement: Supplementary file 5 [file 3-5.pdf]

## Retrosynthesis Route Preview

Compound Illustration: ■ Known ■ Novel

by qihan@accutarbio.com

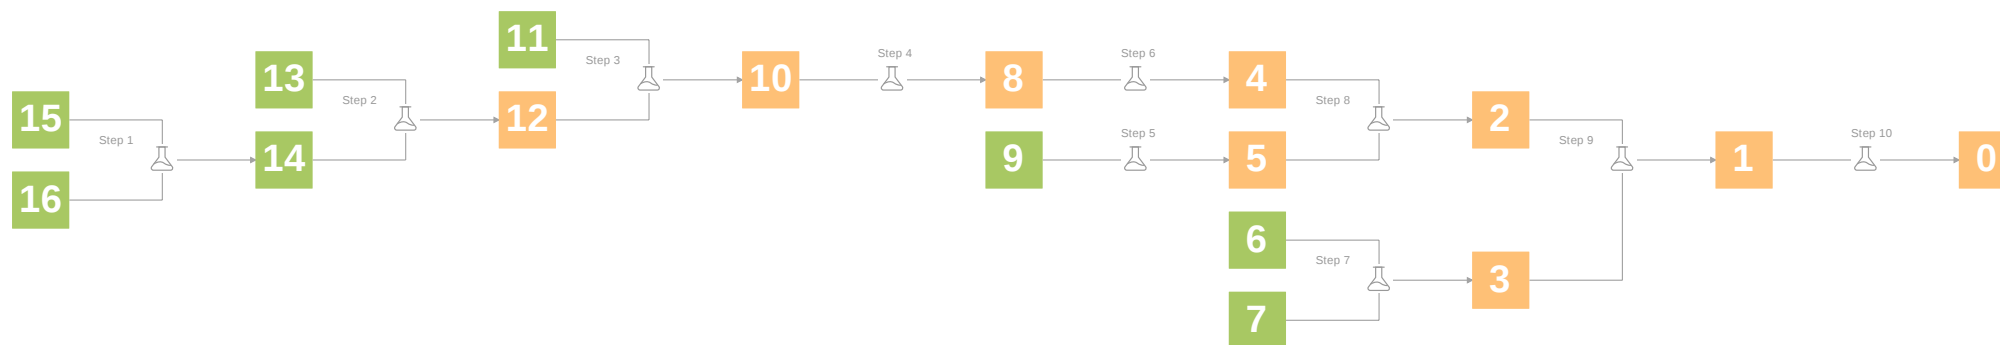

# Route Detail

Compound Illustration: ■ Known ■ Novel

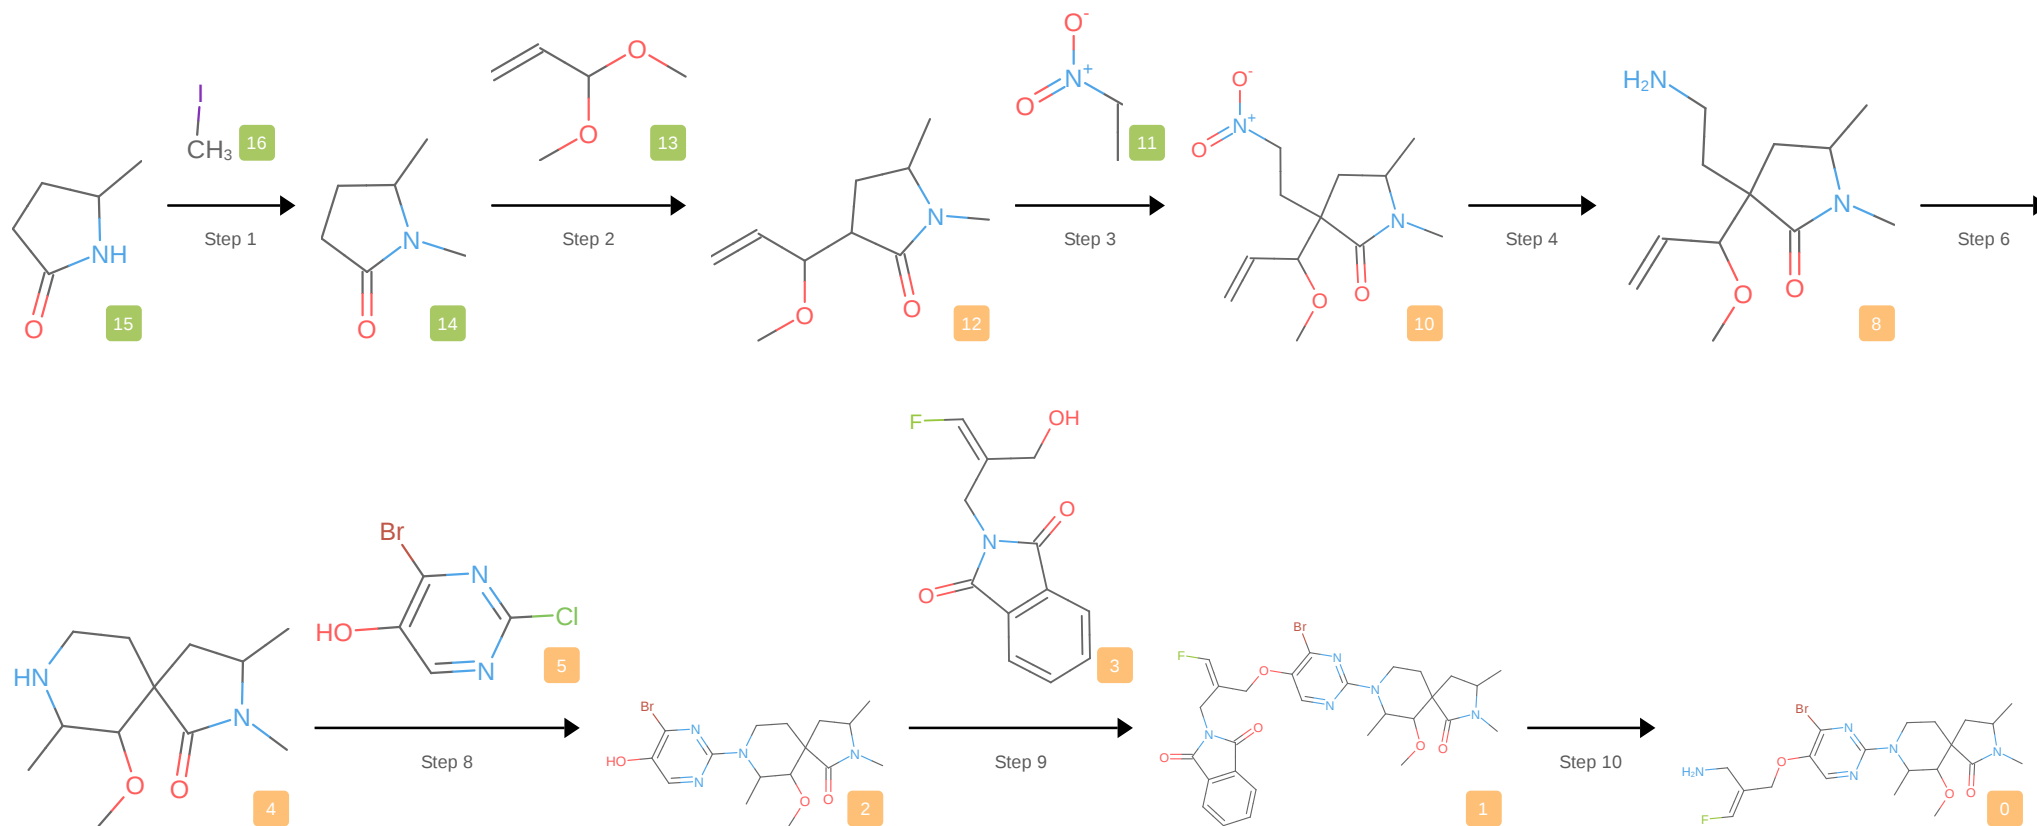

## Route Detail

Compound Illustration: ■ Known ■ Novel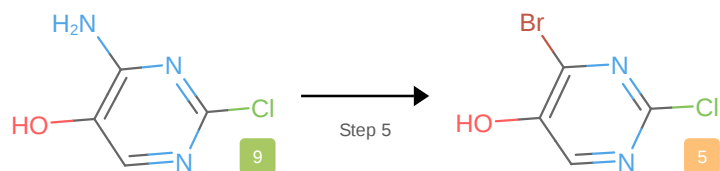

## Route Detail

Compound Illustration: ■ Known ■ Novel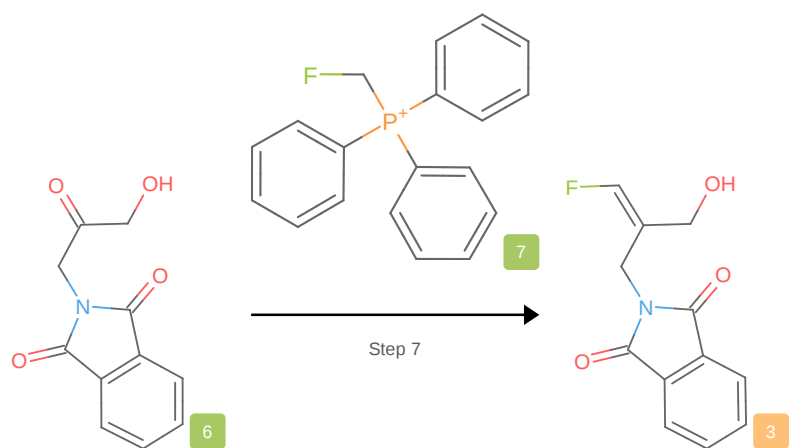

## Step Detail

Compound Illustration: ■ Known ■ Novel

### ◆ Step 1

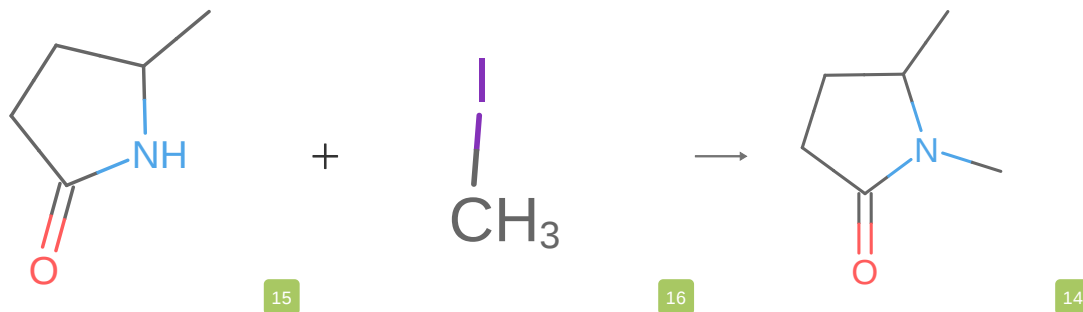

### ◆ Compound Detail

| Reactants Number | Molecular Formula                | Molecular Weight | CAS Number |            |          | PubChem CID |          |          |
|------------------|----------------------------------|------------------|------------|------------|----------|-------------|----------|----------|
| 15               | C <sub>5</sub> H <sub>9</sub> NO | 99.13 g/mol      | 108-27-0   | 62069-49-2 |          | 66055       | 17991654 | 19889147 |
| 16               | CH <sub>3</sub> I                | 141.93 g/mol     | 74-88-4    | 751-82-6   | 865-43-0 | 6328        | 32173    | 58265    |

| Product Number | Molecular Formula                 | Molecular Weight | CAS Number |  |  | PubChem CID |          |          |
|----------------|-----------------------------------|------------------|------------|--|--|-------------|----------|----------|
| 14             | C <sub>6</sub> H <sub>11</sub> NO | 113.16 g/mol     | 5075-92-3  |  |  | 101194      | 17991654 | 67790390 |

### ◆ Reaction Condition

|           |                                         |
|-----------|-----------------------------------------|
| Condition | sodium hydride, tetrahydrofuran.        |
| Condition | sodium hydride, N,N-dimethyl-formamide. |
| Condition | sodium hydride.                         |

## Step Detail

Compound Illustration: ■ Known ■ Novel

### ◆ Step 2

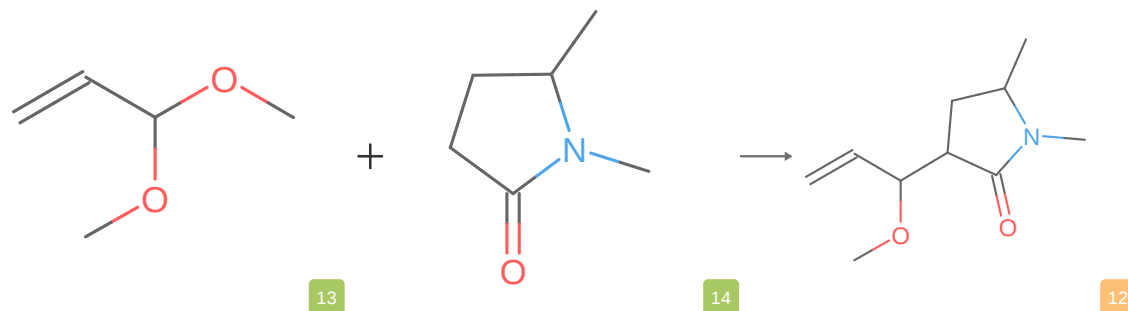

### ◆ Compound Detail

| Reactants Number | Molecular Formula                             | Molecular Weight | CAS Number | PubChem CID              |
|------------------|-----------------------------------------------|------------------|------------|--------------------------|
| 13               | C <sub>5</sub> H <sub>10</sub> O <sub>2</sub> | 102.13 g/mol     | 6044-68-4  | 80145 11137115 20441113  |
| 14               | C <sub>6</sub> H <sub>11</sub> NO             | 113.16 g/mol     | 5075-92-3  | 101194 17991654 67790390 |

| Product Number | Molecular Formula                               | Molecular Weight | CAS Number | PubChem CID |
|----------------|-------------------------------------------------|------------------|------------|-------------|
| 12             | C <sub>10</sub> H <sub>17</sub> NO <sub>2</sub> | 183.25 g/mol     |            |             |

### ◆ Reaction Condition

|           |                                                                                                            |
|-----------|------------------------------------------------------------------------------------------------------------|
| Condition | trimethylsilyl trifluoromethanesulfonate, N-ethyl-N,N-diisopropylamine, dichloromethane.                   |
| Condition | titanium tetrachloride, N-ethyl-N,N-diisopropylamine, boron trifluoride diethyl etherate, dichloromethane. |
| Condition | tetrakis(triphenylphosphine) palladium(0), tetrahydrofuran.                                                |

## Step Detail

Compound Illustration: ■ Known ■ Novel

### ◆ Step 3

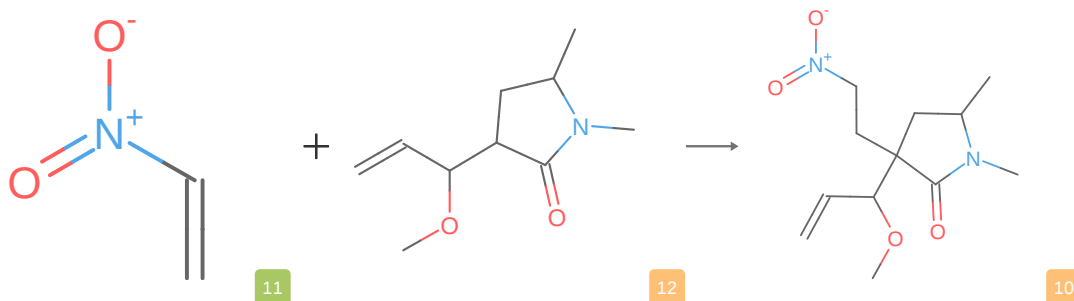

### ◆ Compound Detail

| Reactants Number | Molecular Formula                               | Molecular Weight | CAS Number                       | PubChem CID            |
|------------------|-------------------------------------------------|------------------|----------------------------------|------------------------|
| 11               | C <sub>2</sub> H <sub>3</sub> NO <sub>2</sub>   | 73.05 g/mol      | 3638-64-0 26618-70-2 827022-94-6 | 77197 6713467 18340010 |
| 12               | C <sub>10</sub> H <sub>17</sub> NO <sub>2</sub> | 183.25 g/mol     |                                  |                        |

| Product Number | Molecular Formula                                             | Molecular Weight | CAS Number | PubChem CID |
|----------------|---------------------------------------------------------------|------------------|------------|-------------|
| 10             | C <sub>12</sub> H <sub>20</sub> N <sub>2</sub> O <sub>4</sub> | 256.30 g/mol     |            |             |

### ◆ Reaction Condition

|           |                                                                       |
|-----------|-----------------------------------------------------------------------|
| Condition | lithium diisopropyl amide, tetrahydrofuran.                           |
| Condition | ethyl acetate, toluene.                                               |
| Condition | diisopropylamine, lithium diisopropyl amide, tetrahydrofuran, hexane. |

## Step Detail

Compound Illustration: ■ Known ■ Novel

### ◆ Step 4

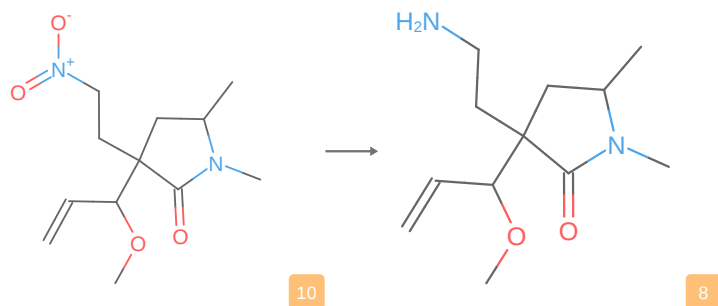

### ◆ Compound Detail

| Reactants Number | Molecular Formula                                             | Molecular Weight | CAS Number | PubChem CID |
|------------------|---------------------------------------------------------------|------------------|------------|-------------|
| 10               | C <sub>12</sub> H <sub>20</sub> N <sub>2</sub> O <sub>4</sub> | 256.30 g/mol     |            |             |

| Product Number | Molecular Formula                                             | Molecular Weight | CAS Number | PubChem CID |
|----------------|---------------------------------------------------------------|------------------|------------|-------------|
| 8              | C <sub>12</sub> H <sub>22</sub> N <sub>2</sub> O <sub>2</sub> | 226.32 g/mol     |            |             |

### ◆ Reaction Condition

|           |                   |
|-----------|-------------------|
| Condition | nickel, ethanol.  |
| Condition | nickel, methanol. |
| Condition | methanol.         |



## Step Detail

Compound Illustration: ■ Known ■ Novel

## ◆ Step 5

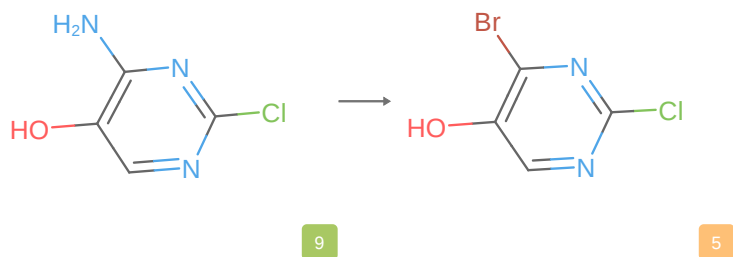

## ◆ Compound Detail

| Reactants Number | Molecular Formula                                | Molecular Weight | CAS Number  | PubChem CID |
|------------------|--------------------------------------------------|------------------|-------------|-------------|
| 9                | C <sub>4</sub> H <sub>4</sub> N <sub>3</sub> OCl | 145.55 g/mol     | 943995-31-1 | 86634908    |

| Product Number | Molecular Formula                                  | Molecular Weight | CAS Number | PubChem CID |
|----------------|----------------------------------------------------|------------------|------------|-------------|
| 5              | C <sub>4</sub> H <sub>2</sub> N <sub>2</sub> OClBr | 209.43 g/mol     |            |             |

## ◆ Reaction Condition

| Condition | sodium nitrite, sodium disulfite, sodium hydroxide, copper(II) bromide. |
|-----------|-------------------------------------------------------------------------|
| Condition | tert.-butylnitrite, copper(II) bromide, acetonitrile.                   |
| Condition | copper(II) bromide, isopentyl nitrite, acetonitrile.                    |

## Step Detail

Compound Illustration: ■ Known ■ Novel

## ◆ Step 6

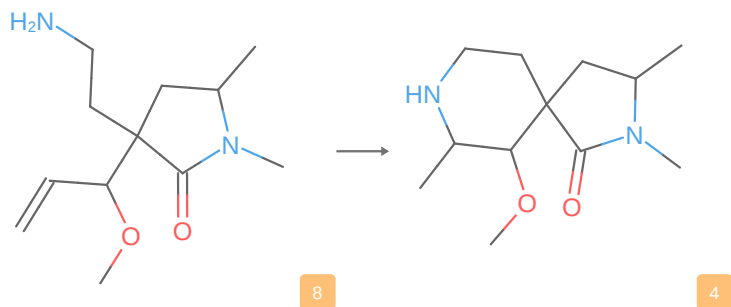

## ◆ Compound Detail

| Reactants Number | Molecular Formula                                             | Molecular Weight | CAS Number | PubChem CID |
|------------------|---------------------------------------------------------------|------------------|------------|-------------|
| 8                | C <sub>12</sub> H <sub>22</sub> N <sub>2</sub> O <sub>2</sub> | 226.32 g/mol     |            |             |

| Product Number | Molecular Formula                                             | Molecular Weight | CAS Number | PubChem CID |
|----------------|---------------------------------------------------------------|------------------|------------|-------------|
| 4              | C <sub>12</sub> H <sub>22</sub> N <sub>2</sub> O <sub>2</sub> | 226.32 g/mol     |            |             |

## ◆ Reaction Condition

| Condition | toluene.       |
|-----------|----------------|
| Condition | (2)H8-toluene. |
| Condition | benzene.       |

## Step Detail

Compound Illustration: ■ Known ■ Novel

### ◆ Step 7

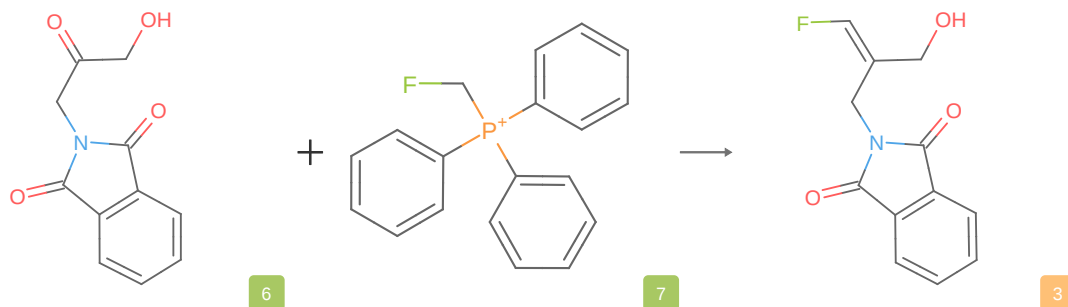

### ◆ Compound Detail

| Reactants Number | Molecular Formula                              | Molecular Weight | CAS Number | PubChem CID                |
|------------------|------------------------------------------------|------------------|------------|----------------------------|
| 6                | C <sub>11</sub> H <sub>9</sub> NO <sub>4</sub> | 219.20 g/mol     | 35750-04-0 | 12104842                   |
| 7                | C <sub>19</sub> H <sub>17</sub> FP             | 295.32 g/mol     | 96385-23-8 | 11303586 11303587 85536740 |

| Product Number | Molecular Formula                                 | Molecular Weight | CAS Number | PubChem CID |
|----------------|---------------------------------------------------|------------------|------------|-------------|
| 3              | C <sub>12</sub> H <sub>10</sub> NO <sub>3</sub> F | 235.21 g/mol     |            |             |

### ◆ Reaction Condition

|           |                                                                      |
|-----------|----------------------------------------------------------------------|
| Condition | sodium hexamethyldisilazane, tetrahydrofuran, tetrafluoroboric acid. |
| Condition | sodium hexamethyldisilazane, tetrahydrofuran, tetrahydrofuran.       |
| Condition | hydrogen iodide.                                                     |

## Step Detail

Compound Illustration: ■ Known ■ Novel

### ◆ Step 8

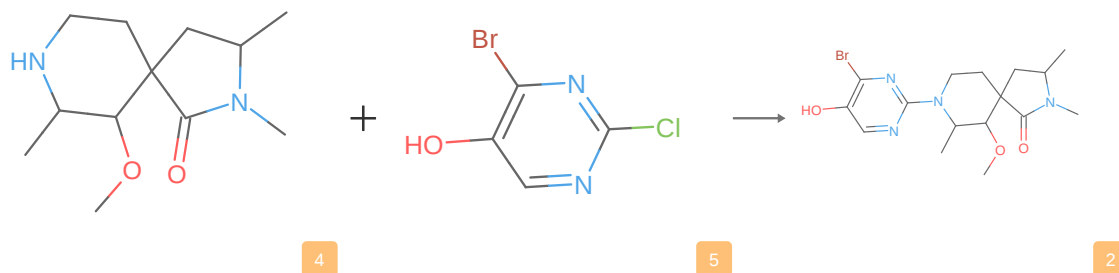

### ◆ Compound Detail

| Reactants Number | Molecular Formula                                             | Molecular Weight | CAS Number | PubChem CID |
|------------------|---------------------------------------------------------------|------------------|------------|-------------|
| 4                | C <sub>12</sub> H <sub>22</sub> N <sub>2</sub> O <sub>2</sub> | 226.32 g/mol     |            |             |
| 5                | C <sub>4</sub> H <sub>2</sub> N <sub>2</sub> OCIBr            | 209.43 g/mol     |            |             |

| Product Number | Molecular Formula                                                | Molecular Weight | CAS Number | PubChem CID |
|----------------|------------------------------------------------------------------|------------------|------------|-------------|
| 2              | C <sub>16</sub> H <sub>23</sub> N <sub>4</sub> O <sub>3</sub> Br | 399.29 g/mol     |            |             |

### ◆ Reaction Condition

| Condition | methanol, sodium hydrogencarbonate, ethylene glycol, ethyl acetate. |
|-----------|---------------------------------------------------------------------|
| Condition | NaHCO <sub>3</sub> , ethylene glycol.                               |
| Condition | ethanol.                                                            |

## Step Detail

Compound Illustration: ■ Known ■ Novel

### ◆ Step 9

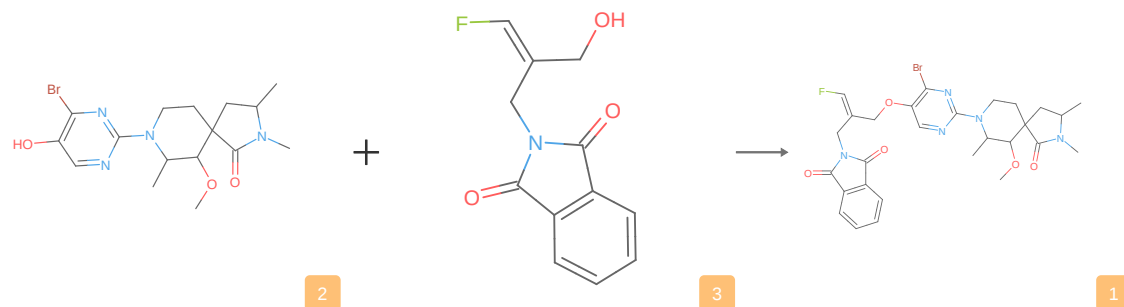

### ◆ Compound Detail

| Reactants Number | Molecular Formula                                                | Molecular Weight | CAS Number | PubChem CID |
|------------------|------------------------------------------------------------------|------------------|------------|-------------|
| 2                | C <sub>16</sub> H <sub>23</sub> N <sub>4</sub> O <sub>3</sub> Br | 399.29 g/mol     |            |             |
| 3                | C <sub>12</sub> H <sub>10</sub> NO <sub>3</sub> F                | 235.21 g/mol     |            |             |

| Product Number | Molecular Formula                                                 | Molecular Weight | CAS Number | PubChem CID |
|----------------|-------------------------------------------------------------------|------------------|------------|-------------|
| 1              | C <sub>28</sub> H <sub>31</sub> N <sub>5</sub> O <sub>5</sub> FBr | 616.48 g/mol     |            |             |

### ◆ Reaction Condition

|           |                                                                        |
|-----------|------------------------------------------------------------------------|
| Condition | di-isopropyl azodicarboxylate, triphenylphosphine, tetrahydrofuran.    |
| Condition | triphenylphosphine, diethylazodicarboxylate, tetrahydrofuran, toluene. |
| Condition | tributylphosphine, 1,1'-azodicarbonyl-dipiperidine, tetrahydrofuran.   |

## Step Detail

Compound Illustration: ■ Known ■ Novel

### ◆ Step 10

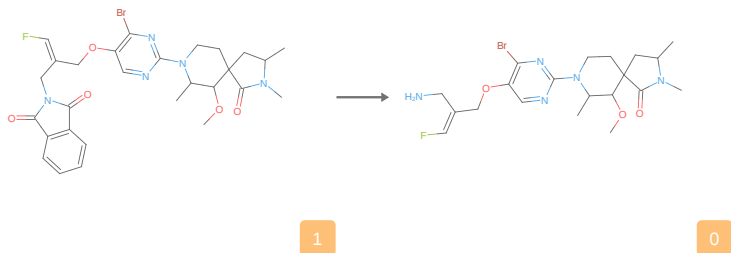

### ◆ Compound Detail

| Reactants Number | Molecular Formula                                                 | Molecular Weight | CAS Number | PubChem CID |
|------------------|-------------------------------------------------------------------|------------------|------------|-------------|
| 1                | C <sub>28</sub> H <sub>31</sub> N <sub>5</sub> O <sub>5</sub> FBr | 616.48 g/mol     |            |             |

| Product Number | Molecular Formula                                                 | Molecular Weight | CAS Number | PubChem CID |
|----------------|-------------------------------------------------------------------|------------------|------------|-------------|
| 0              | C <sub>20</sub> H <sub>29</sub> N <sub>5</sub> O <sub>3</sub> FBr | 486.38 g/mol     |            |             |

### ◆ Reaction Condition

|           |                              |
|-----------|------------------------------|
| Condition | hydrazine, methanol.         |
| Condition | hydrazine hydrate, methanol. |
| Condition | hydrazine.                   |
