# Supplementary material for: ChemiRise: a data-driven retrosynthesis engine
Source: arXiv:2108.04682 ancillary file (2021-08-09)
Supplement: Supplementary file 6 [file 3-6.pdf]

## Retrosynthesis Route Preview

Compound Illustration: ■ Known ■ Novel

by qihan@accutarbio.com

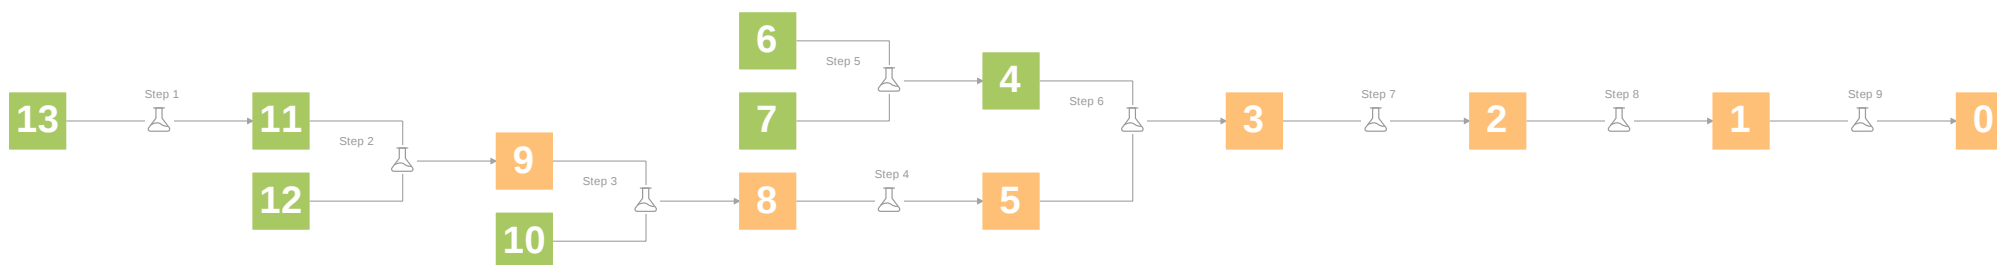

# Route Detail

Compound Illustration: ■ Known ■ Novel

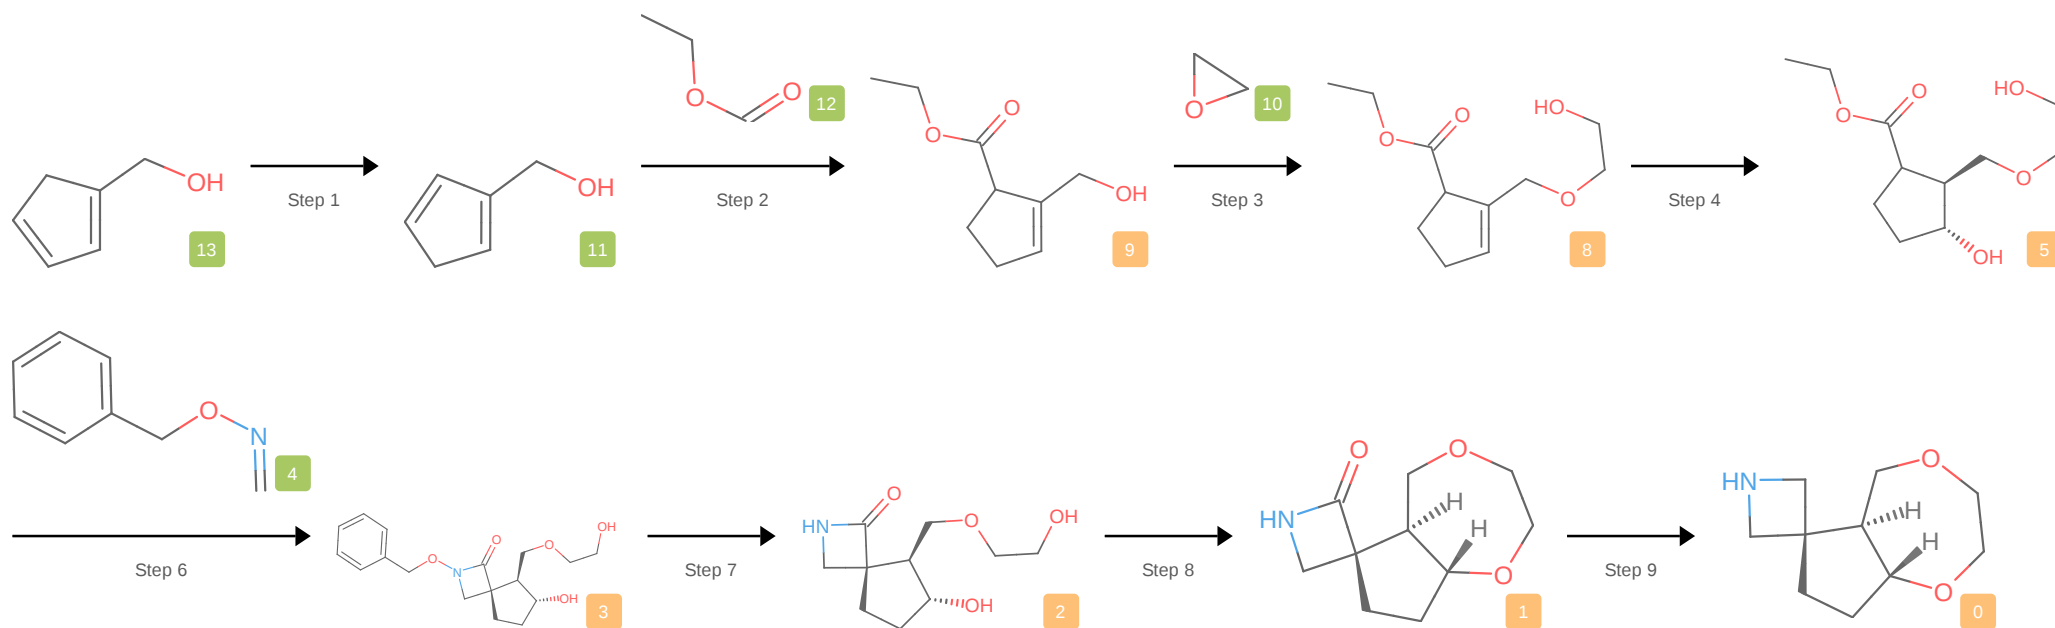

## Route Detail

Compound Illustration: ■ Known ■ Novel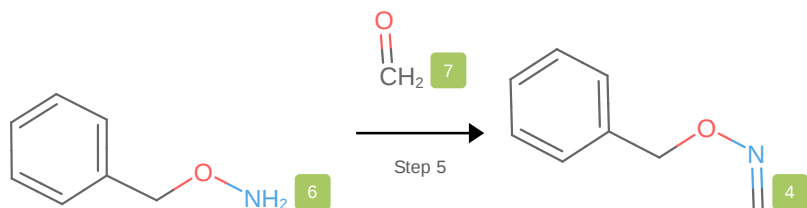

## Step Detail

Compound Illustration: ■ Known ■ Novel

### ◆ Step 1

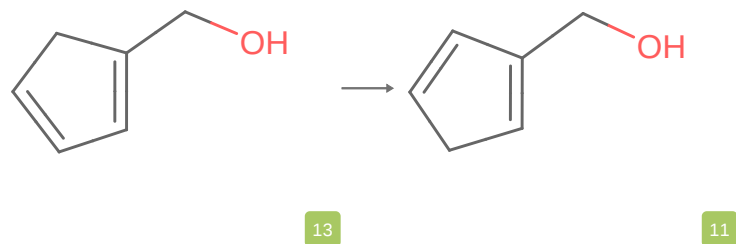

### ◆ Compound Detail

| Reactants Number | Molecular Formula               | Molecular Weight | CAS Number | PubChem CID              |
|------------------|---------------------------------|------------------|------------|--------------------------|
| 13               | C <sub>6</sub> H <sub>8</sub> O | 96.13 g/mol      | 1273-86-5  | 2777811 2777812 10601634 |

| Product Number | Molecular Formula               | Molecular Weight | CAS Number | PubChem CID        |
|----------------|---------------------------------|------------------|------------|--------------------|
| 11             | C <sub>6</sub> H <sub>8</sub> O | 96.13 g/mol      |            | 15535273 101262990 |

### ◆ Reaction Condition

|           |                                                                     |
|-----------|---------------------------------------------------------------------|
| Condition | triethylamine.                                                      |
| Condition | ethanol.                                                            |
| Condition | potassium tert-butyrate, N,N,N,N,N,N-hexamethylphosphoric triamide. |

## Step Detail

Compound Illustration: ■ Known ■ Novel

### ◆ Step 2

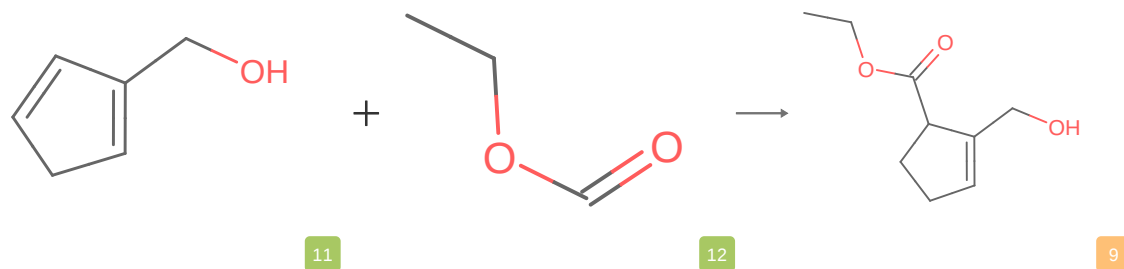

### ◆ Compound Detail

| Reactants Number | Molecular Formula                            | Molecular Weight | CAS Number |            |             | PubChem CID |           |         |
|------------------|----------------------------------------------|------------------|------------|------------|-------------|-------------|-----------|---------|
| 11               | C <sub>6</sub> H <sub>8</sub> O              | 96.13 g/mol      |            |            |             | 15535273    | 101262990 |         |
| 12               | C <sub>3</sub> H <sub>6</sub> O <sub>2</sub> | 74.08 g/mol      | 109-94-4   | 35976-76-2 | 167614-38-2 | 8025        | 142039    | 6914132 |

| Product Number | Molecular Formula                             | Molecular Weight | CAS Number |  |  | PubChem CID |  |  |
|----------------|-----------------------------------------------|------------------|------------|--|--|-------------|--|--|
| 9              | C <sub>9</sub> H <sub>14</sub> O <sub>3</sub> | 170.21 g/mol     |            |  |  |             |  |  |

### ◆ Reaction Condition

|           |                                        |
|-----------|----------------------------------------|
| Condition | toluene.                               |
| Condition | acetone.                               |
| Condition | dodecacarbonyl-triangulo-triruthenium. |

## Step Detail

Compound Illustration: ■ Known ■ Novel

### ◆ Step 3

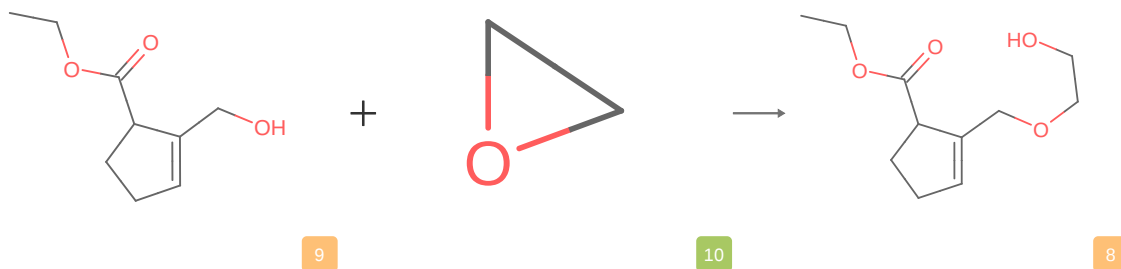

### ◆ Compound Detail

| Reactants Number | Molecular Formula                             | Molecular Weight | CAS Number |           |           | PubChem CID |       |       |
|------------------|-----------------------------------------------|------------------|------------|-----------|-----------|-------------|-------|-------|
| 9                | C <sub>9</sub> H <sub>14</sub> O <sub>3</sub> | 170.21 g/mol     |            |           |           |             |       |       |
| 10               | C <sub>2</sub> H <sub>4</sub> O               | 44.05 g/mol      | 75-21-8    | 6552-57-4 | 8070-50-6 | 6354        | 24751 | 61429 |

| Product Number | Molecular Formula                              | Molecular Weight | CAS Number |  |  | PubChem CID |  |  |
|----------------|------------------------------------------------|------------------|------------|--|--|-------------|--|--|
| 8              | C <sub>11</sub> H <sub>18</sub> O <sub>4</sub> | 214.26 g/mol     |            |  |  |             |  |  |

### ◆ Reaction Condition

|           |                                     |
|-----------|-------------------------------------|
| Condition | sulfuric acid.                      |
| Condition | sodium hydride.                     |
| Condition | boron trifluoride diethyl etherate. |

## Step Detail

Compound Illustration: ■ Known ■ Novel

### ◆ Step 4

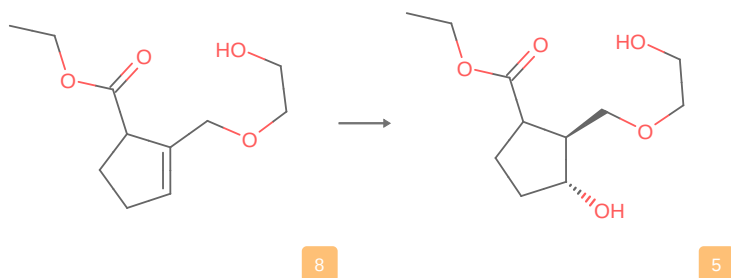

### ◆ Compound Detail

| Reactants Number | Molecular Formula                              | Molecular Weight | CAS Number | PubChem CID |
|------------------|------------------------------------------------|------------------|------------|-------------|
| 8                | C <sub>11</sub> H <sub>18</sub> O <sub>4</sub> | 214.26 g/mol     |            |             |

| Product Number | Molecular Formula                              | Molecular Weight | CAS Number | PubChem CID |
|----------------|------------------------------------------------|------------------|------------|-------------|
| 5              | C <sub>11</sub> H <sub>20</sub> O <sub>5</sub> | 232.27 g/mol     |            |             |

### ◆ Reaction Condition

|           |                                                                     |
|-----------|---------------------------------------------------------------------|
| Condition | borane-THF, dihydrogen peroxide, sodium hydroxide, tetrahydrofuran. |
| Condition | borane-THF, sodium hydroxide, dihydrogen peroxide, tetrahydrofuran. |
| Condition | dihydrogen peroxide, sodium hydroxide, tetrahydrofuran.             |

## Step Detail

Compound Illustration: ■ Known ■ Novel

### ◆ Step 5

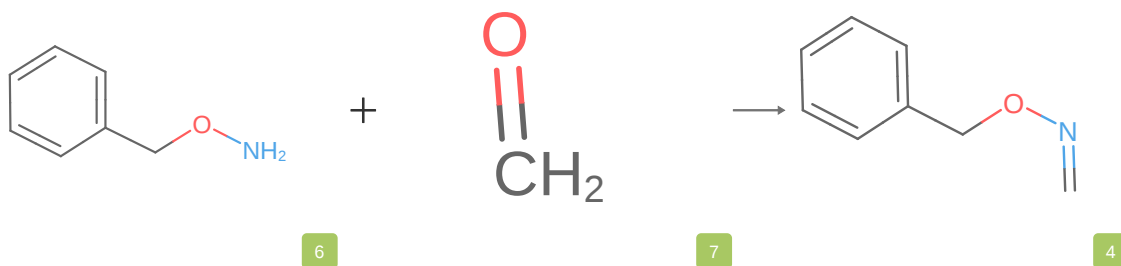

### ◆ Compound Detail

| Reactants Number | Molecular Formula                | Molecular Weight | CAS Number |           |            | PubChem CID |        |         |
|------------------|----------------------------------|------------------|------------|-----------|------------|-------------|--------|---------|
| 6                | C <sub>7</sub> H <sub>9</sub> NO | 123.15 g/mol     | 622-33-3   | 2687-43-6 | 92165-14-5 | 102312      | 102313 | 3499125 |
| 7                | CH <sub>2</sub> O                | 30.03 g/mol      | 50-00-0    | 1336-63-6 | 1664-98-8  | 712         | 25049  | 33268   |

| Product Number | Molecular Formula                | Molecular Weight | CAS Number |  | PubChem CID     |  |
|----------------|----------------------------------|------------------|------------|--|-----------------|--|
| 4              | C <sub>8</sub> H <sub>9</sub> NO | 135.17 g/mol     | 72399-18-9 |  | 561610 88329704 |  |

### ◆ Reaction Condition

|           |           |
|-----------|-----------|
| Condition | methanol. |
| Condition | ethanol.  |
| Condition | water.    |



## Step Detail

Compound Illustration: ■ Known ■ Novel

### ◆ Step 6

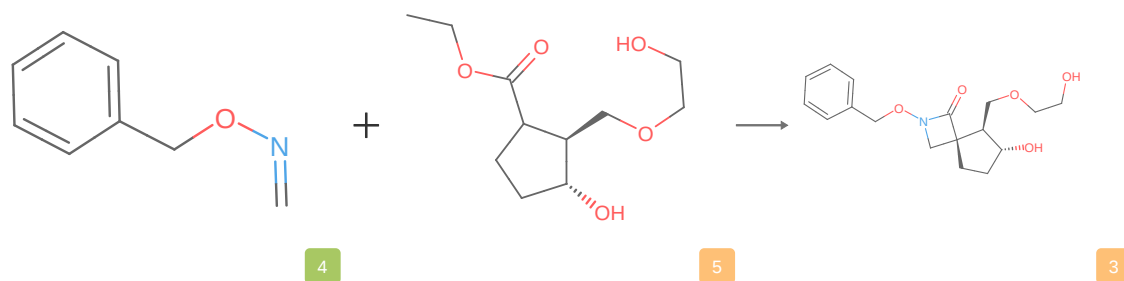

### ◆ Compound Detail

| Reactants Number | Molecular Formula                              | Molecular Weight | CAS Number | PubChem CID     |
|------------------|------------------------------------------------|------------------|------------|-----------------|
| 4                | C <sub>8</sub> H <sub>9</sub> NO               | 135.17 g/mol     | 72399-18-9 | 561610 88329704 |
| 5                | C <sub>11</sub> H <sub>20</sub> O <sub>5</sub> | 232.27 g/mol     |            |                 |

| Product Number | Molecular Formula                               | Molecular Weight | CAS Number | PubChem CID |
|----------------|-------------------------------------------------|------------------|------------|-------------|
| 3              | C <sub>17</sub> H <sub>23</sub> NO <sub>5</sub> | 321.37 g/mol     |            |             |

### ◆ Reaction Condition

|           |                                             |
|-----------|---------------------------------------------|
| Condition | lithium diisopropyl amide.                  |
| Condition | lithium diisopropyl amide, tetrahydrofuran. |
| Condition | n-butyllithium, diisopropylamine.           |

## Step Detail

Compound Illustration: ■ Known ■ Novel

### ◆ Step 7

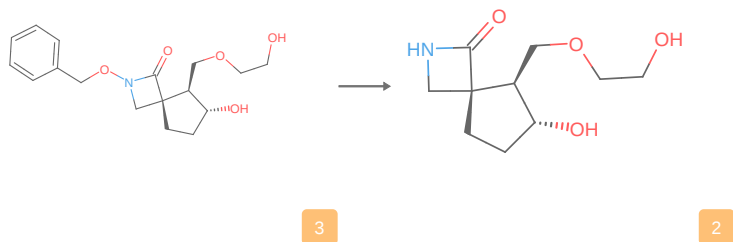

### ◆ Compound Detail

| Reactants Number | Molecular Formula                               | Molecular Weight | CAS Number | PubChem CID |
|------------------|-------------------------------------------------|------------------|------------|-------------|
| 3                | C <sub>17</sub> H <sub>23</sub> NO <sub>5</sub> | 321.37 g/mol     |            |             |

| Product Number | Molecular Formula                               | Molecular Weight | CAS Number | PubChem CID |
|----------------|-------------------------------------------------|------------------|------------|-------------|
| 2              | C <sub>10</sub> H <sub>17</sub> NO <sub>4</sub> | 215.25 g/mol     |            |             |

### ◆ Reaction Condition

|           |                                            |
|-----------|--------------------------------------------|
| Condition | water, nickel.                             |
| Condition | samarium diiodide, tetrahydrofuran, water. |
| Condition | methanol.                                  |

## Step Detail

Compound Illustration: ■ Known ■ Novel

### ◆ Step 8

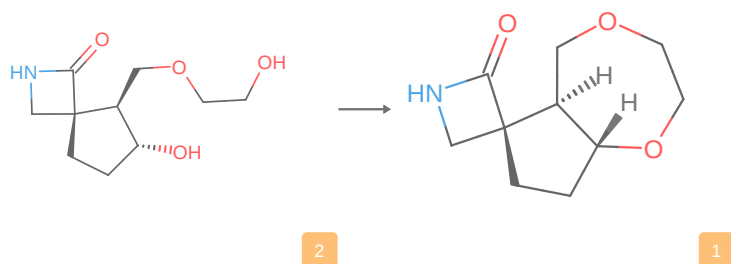

### ◆ Compound Detail

| Reactants Number | Molecular Formula                               | Molecular Weight | CAS Number | PubChem CID |
|------------------|-------------------------------------------------|------------------|------------|-------------|
| 2                | C <sub>10</sub> H <sub>17</sub> NO <sub>4</sub> | 215.25 g/mol     |            |             |

| Product Number | Molecular Formula                               | Molecular Weight | CAS Number | PubChem CID |
|----------------|-------------------------------------------------|------------------|------------|-------------|
| 1              | C <sub>10</sub> H <sub>15</sub> NO <sub>3</sub> | 197.23 g/mol     |            |             |

### ◆ Reaction Condition

|           |                                                                                                                   |
|-----------|-------------------------------------------------------------------------------------------------------------------|
| Condition | toluene-4-sulfonic acid, sodium hydrogencarbonate, toluene, water, ethyl acetate.                                 |
| Condition | dicobalt octacarbonyl, boron trifluoride diethyl etherate, ammonium cerium(IV) nitrate, dichloromethane, acetone. |
| Condition | potassium hydroxide, p-toluenesulfonyl chloride, 1,4-dioxane.                                                     |

## Step Detail

Compound Illustration: ■ Known ■ Novel

### ◆ Step 9

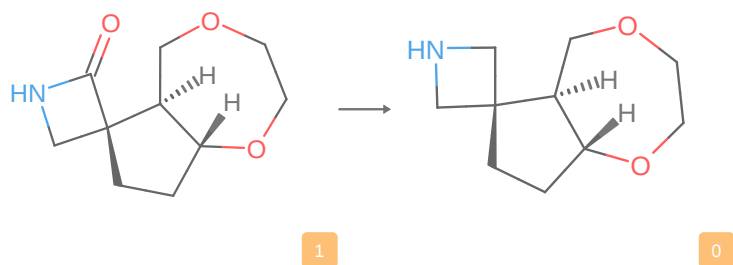

### ◆ Compound Detail

| Reactants Number | Molecular Formula                               | Molecular Weight | CAS Number | PubChem CID |
|------------------|-------------------------------------------------|------------------|------------|-------------|
| 1                | C <sub>10</sub> H <sub>15</sub> NO <sub>3</sub> | 197.23 g/mol     |            |             |

| Product Number | Molecular Formula                               | Molecular Weight | CAS Number | PubChem CID |
|----------------|-------------------------------------------------|------------------|------------|-------------|
| 0              | C <sub>10</sub> H <sub>17</sub> NO <sub>2</sub> | 183.25 g/mol     |            |             |

### ◆ Reaction Condition

|           |                                                  |
|-----------|--------------------------------------------------|
| Condition | lithium aluminium tetrahydride, diethyl ether.   |
| Condition | tetrahydrofuran.                                 |
| Condition | lithium aluminium tetrahydride, tetrahydrofuran. |
