# Supplementary material for: ChemiRise: a data-driven retrosynthesis engine
Source: arXiv:2108.04682 ancillary file (2021-08-09)
Supplement: Supplementary file 7 [file 3-7.pdf]

## Retrosynthesis Route Preview

Compound Illustration: ■ Known ■ Novel

by qihan@accutarbio.com

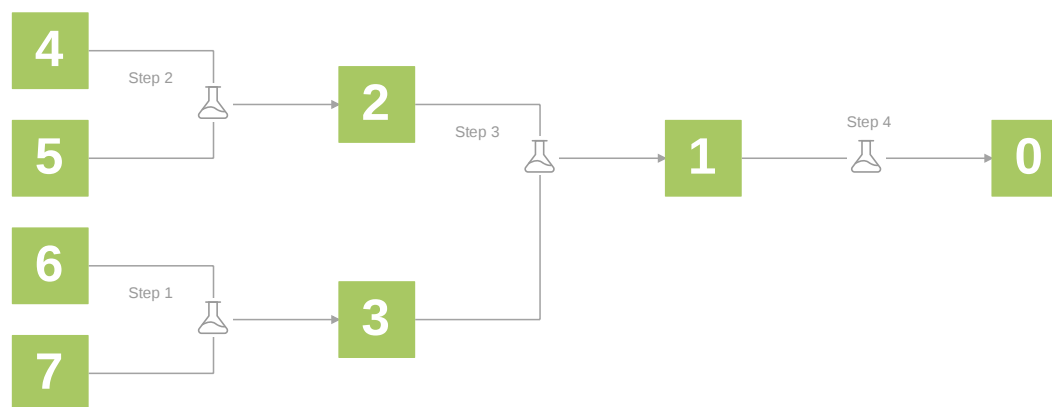

## Route Detail

Compound Illustration: ■ Known ■ Novel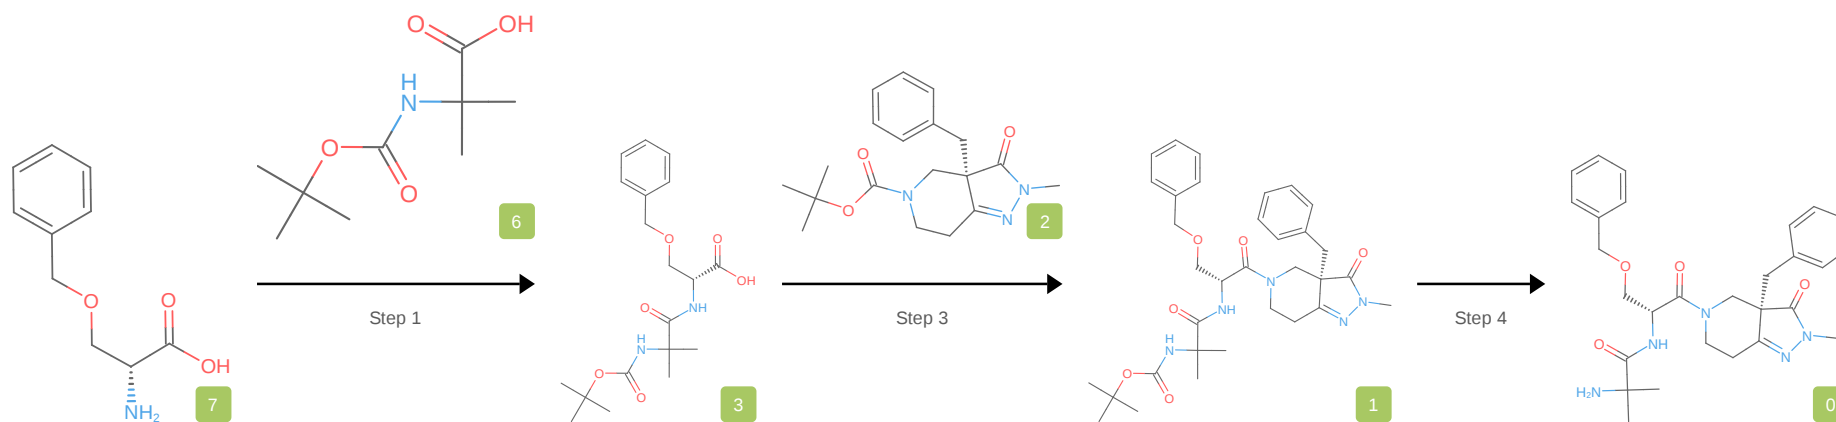

## Route Detail

Compound Illustration: ■ Known ■ Novel

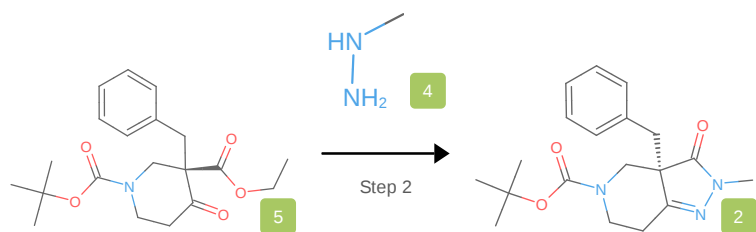

## Step Detail

Compound Illustration: ■ Known ■ Novel

### ◆ Step 1

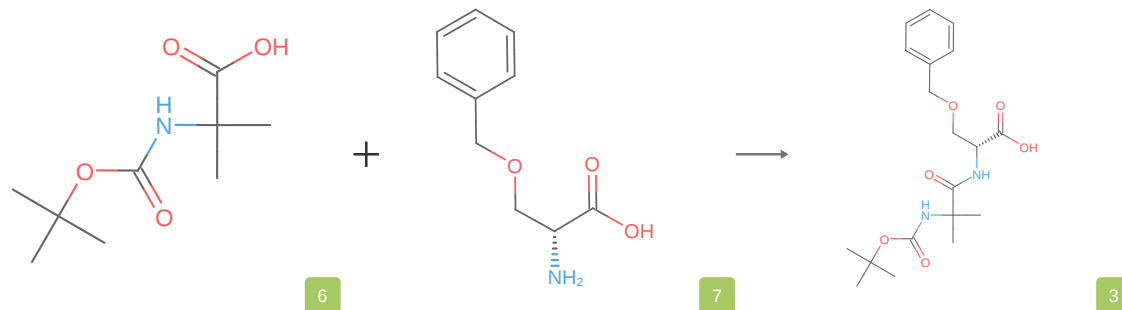

### ◆ Compound Detail

| Reactants Number | Molecular Formula                               | Molecular Weight | CAS Number |              |  | PubChem CID |         |          |
|------------------|-------------------------------------------------|------------------|------------|--------------|--|-------------|---------|----------|
| 6                | C <sub>9</sub> H <sub>17</sub> NO <sub>4</sub>  | 203.24 g/mol     | 30992-29-1 | 52162-92-2   |  | 2733845     | 7004985 | 23677257 |
| 7                | C <sub>10</sub> H <sub>13</sub> NO <sub>3</sub> | 195.22 g/mol     | 10433-52-0 | 1233494-98-8 |  | 112114      | 6950863 | 53229898 |

| Product Number | Molecular Formula                                             | Molecular Weight | CAS Number  |             |              | PubChem CID |          |
|----------------|---------------------------------------------------------------|------------------|-------------|-------------|--------------|-------------|----------|
| 3              | C <sub>19</sub> H <sub>28</sub> N <sub>2</sub> O <sub>6</sub> | 380.44 g/mol     | 159634-89-6 | 159634-89-6 | 1026088-60-7 | 10894202    | 12967000 |

### ◆ Reaction Condition

|           |                                                             |
|-----------|-------------------------------------------------------------|
| Condition | benzotriazol-1-ol, dichloromethane.                         |
| Condition | N-ethyl-N,N-diisopropylamine, N,N-dimethyl-formamide.       |
| Condition | N-ethyl-N,N-diisopropylamine, HATU, N,N-dimethyl-formamide. |

Step Detail

Compound Illustration: Known Novel

Step 2

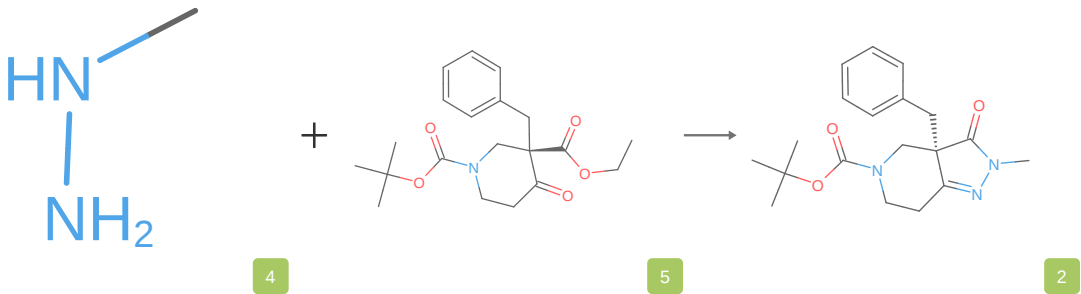

Compound Detail

| Reactants Number | Molecular Formula                               | Molecular Weight | CAS Number  |          |           | PubChem CID       |      |       |
|------------------|-------------------------------------------------|------------------|-------------|----------|-----------|-------------------|------|-------|
| 4                | CH <sub>6</sub> N <sub>2</sub>                  | 46.07 g/mol      | 60-34-4     | 302-15-8 | 5118-34-3 | 6061              | 9323 | 34664 |
| 5                | C <sub>20</sub> H <sub>27</sub> NO <sub>5</sub> | 361.44 g/mol     | 219324-21-7 |          |           | 25258320 54130376 |      |       |

| Product Number | Molecular Formula                                             | Molecular Weight | CAS Number  |  | PubChem CID       |  |
|----------------|---------------------------------------------------------------|------------------|-------------|--|-------------------|--|
| 2              | C <sub>19</sub> H <sub>25</sub> N <sub>3</sub> O <sub>3</sub> | 343.42 g/mol     | 193274-02-1 |  | 54036273 11961928 |  |

Reaction Condition

|           |                                  |
|-----------|----------------------------------|
| Condition | toluene.                         |
| Condition | ethanol.                         |
| Condition | triethylamine, ethanol, ethanol. |

## Step Detail

Compound Illustration: ■ Known ■ Novel

### ◆ Step 3

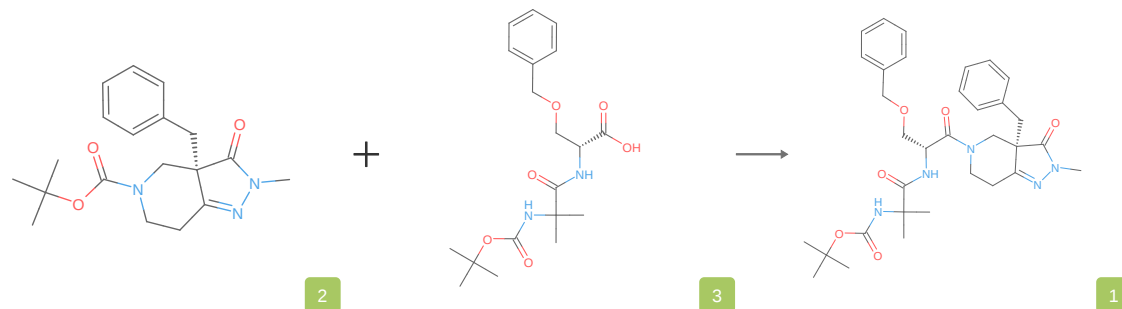

### ◆ Compound Detail

| Reactants Number | Molecular Formula                                             | Molecular Weight | CAS Number                           | PubChem CID       |
|------------------|---------------------------------------------------------------|------------------|--------------------------------------|-------------------|
| 2                | C <sub>19</sub> H <sub>25</sub> N <sub>3</sub> O <sub>3</sub> | 343.42 g/mol     | 193274-02-1                          | 54036273 11961928 |
| 3                | C <sub>19</sub> H <sub>28</sub> N <sub>2</sub> O <sub>6</sub> | 380.44 g/mol     | 159634-89-6 159634-89-6 1026088-60-7 | 10894202 12967000 |

| Product Number | Molecular Formula                                             | Molecular Weight | CAS Number | PubChem CID       |
|----------------|---------------------------------------------------------------|------------------|------------|-------------------|
| 1              | C <sub>33</sub> H <sub>43</sub> N <sub>5</sub> O <sub>6</sub> | 605.73 g/mol     |            | 11238815 69370796 |

### ◆ Reaction Condition

|           |                                                                                                                                                             |
|-----------|-------------------------------------------------------------------------------------------------------------------------------------------------------------|
| Condition | trifluoroacetic acid, N-ethyl-N,N-diisopropylamine, dichloromethane, N,N-dimethyl-formamide.                                                                |
| Condition | hydrogenchloride, N-ethyl-N,N-diisopropylamine, 1,4-dioxane, tetrahydrofuran.                                                                               |
| Condition | hydrogenchloride, N-ethyl-N,N-diisopropylamine, bromo-tris(1-pyrrolidinyl)phosphonium hexafluorophosphate, 1,4-dioxane, chloroform, N,N-dimethyl-formamide. |

Step Detail

Compound Illustration: ■ Known ■ Novel

◆ Step 4

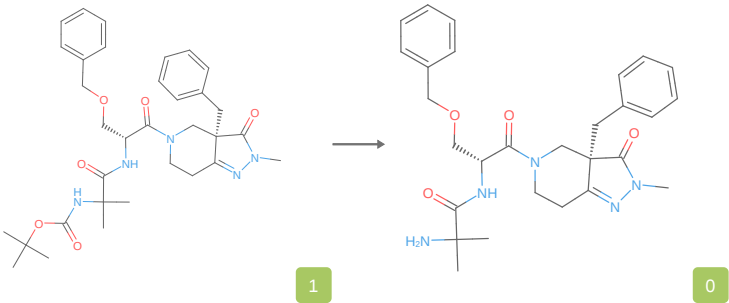

◆ Compound Detail

| Reactants Number | Molecular Formula                                             | Molecular Weight | CAS Number | PubChem CID       |
|------------------|---------------------------------------------------------------|------------------|------------|-------------------|
| 1                | C <sub>33</sub> H <sub>43</sub> N <sub>5</sub> O <sub>6</sub> | 605.73 g/mol     |            | 11238815 69370796 |

| Product Number | Molecular Formula                                             | Molecular Weight | CAS Number                          | PubChem CID            |
|----------------|---------------------------------------------------------------|------------------|-------------------------------------|------------------------|
| 0              | C <sub>28</sub> H <sub>35</sub> N <sub>5</sub> O <sub>4</sub> | 505.62 g/mol     | 193273-66-4 193273-69-7 193273-66-4 | 216208 9852609 9852610 |

◆ Reaction Condition

|           |                                        |
|-----------|----------------------------------------|
| Condition | hydrogenchloride, ethyl acetate.       |
| Condition | dichloromethane, trifluoroacetic acid. |
| Condition | trifluoroacetic acid, dichloromethane. |
